# Supplementary material for: ByteComp: Revisiting Gradient Compression in Distributed Training
Source: arXiv:2205.14465 source file (2022-06-06)
Supplement: Supplementary file 1 [file appendix.tex]

\appendix
\section*{Appendix}

\section{Cost Models of Collective Routines}
\label{app:cost_models}

We first briefly introduce how different collective routines work for gradient synchronization.

\noindent \textbf{Allreduce} combines values from all processes and distributes the results back to all processes.
It is the most frequently used collective operation for the aggregation of gradient updates.

\noindent \textbf{Allgather} gathers data from all processes and distributes its own data to all processes. 
It can be used for the communication of many compression algorithms when the compressed tensors are not allreducible because their aggregation operation is not associative~\cite{xu2021grace, agarwal2021utility}.

\noindent \textbf{Reduce/Broadcast} first reduces values on all processes to the root process, which then broadcasts the results to all other processes.

\noindent \textbf{Reduce-scatter/Allgather} first reduces values across processes with each receiving part of the results. It then uses Allgather to ensure that all processes have the whole results.

\noindent \textbf{Gather/Broadcast} first gathers data from all processes to the root process. Compared to Reduce/Broadcast, it needs to perform some additional operations, such as reduction and compression/decompression if tensors are compressed, before the root process broadcasts the results to all processes.

\noindent \textbf{Alltoall/Allgather} first sends the same amount of data to each other, and receives the same amount of data from each other. Compared to Reduce-scatter/Allgather, it needs to perform some additional operations, such as reduction and compression/decompression if tensors are compressed, before the Allgather operation.

Table~\ref{table:comp_comm_overhead} lists the cost models of both communication and compression time of different collective routines in flat communication.
Let $n$ be the number of nodes, B the network bandwidth, and $M$ the message size on each node after compression. 
The communication time follows the cost model analysis in the literature~\cite{MPIoptimization, broadcast}.

$h_1(\cdot)$ is the compression time and $h_2(\cdot)$ is the decompression time. 
We profile the compression and decompression time offline as a function of $M$ for different compression algorithms with different compute resources, such as GPUs and CPUs.
Given a compression algorithm and compute resource, we measure the operation time with many sampled message sizes, such as $2^{10}, 2^{11}, \cdots, 2^{30}$, and then approximately obtain the cost models with curve fitting.
Overall compression time is the sum of compression time and decompression time.

\begin{table*}[ht!]
\small
\centering
\begin{tabular}{l|l|c|c}
\hline
Communication routines   & Tensor types     & Communication time & Overall compression time \\ \hline \hline
Allreduce               & allreducible tensor     & $\frac{2(n-1)M}{nB}$   &  $h_1(M) + h_2(M) $        \\ \hline
Allgather               & any types & $(n-1)M/B$             & $h_1(M) + nh_2(M)$ \\ \hline
Alltoall/Allgather      & sparse tensor    & $\frac{(n^2-1)M}{nB}$  & $h_1(M) + n^2h_2(M/n)$             \\ \hline
Alltoall/Allgather      & quantized tensor & $\frac{2(n-1)M}{nB}$   & $h_1(M) + h_1(M/n)+2nh_2(M/n)$             \\ \hline
Gather/Broadcast        & sparse tensor   & $(2n-1)M/B$    & $h_1(M) + nh_2(M)$             \\ \hline
Gather/Broadcast        & quantized tensor   & $nM/B$           & $2h_1(M) + (n+1)h_2(M)$             \\
\hline
\end{tabular}

\caption {The cost models of various collective routines in flat communication for compression. $n$ is the number of nodes, B is the network bandwidth, and $M$ is the message size on each node after compression. $h_1(\cdot)$ is the compression time and $h_2(\cdot)$ is the decompression time. Overall compression time is the sum of compression time and decompression time.}
\label{table:comp_comm_overhead}
\vskip -0.2in
\end{table*}

\noindent \textbf{Allreduce.} 
The process is compression, Allreduce, and decompression.
The compression time is $h_1(M)$.
The communication time for Allreduce is $\frac{2(n-1)M}{nB}$. 
Because the tensor is allreducible, the received data is aggregated so that the decompression time is $h_2(M)$. 
The overall compression time is $h_1(M) + h_2(M)$.
Note that Allreduce is also used for the gradient synchronization of FP32 and the overall compression time is 0.

\noindent \textbf{Allgather.} 
The process is compression, Allgather, and decompression.
The compression time is $h_1(M)$.
The communication time for Allgather is $(n-1)M/B$.
There are $n$ compressed tensors received at each node so that there are $n$ decompression operations and the decompression time is $nh_2(M)$.
The overall compression time is $h_1(M) + nh_2(M)$.

\noindent \textbf{Alltoall/Allgather.}
There are two possible processes for compression with Alltoall/Allgather as the communication.
One is compression, Alltoall, Allgather, and decompression.
The compression time is $h_1(M)$.
The communication time for Alltoall is $\frac{(n-1)M}{nB}$.
The tensor size at each node after Alltoall is still $M$ because each node receives $n$ chunks with the size of $M/n$.
Hence, the communication time for Allgather is $(n-1)M/B$.
There are $n^2$ compressed tensors with the size of $M/n$ received at each node after Allgather so that there are $n^2$ decompression operations and the decompression time is $n^2h_2(M/n)$.
The overall compression time is $h_1(M) + n^2h_2(M/n)$ and the overall communication time is $\frac{(n^2-1)M}{nB}$.

The other process is compression, Alltoall, decompression, compression, Allgather, and decompression.
The compression time is $h_1(M)$.
The communication time for Alltoall is $\frac{(n-1)M}{nB}$.
The decompression time after Alltoall is $nh_2(M/n)$.
The second compression can keep the same compression rate, or change it to another one.
Without loss of generality, we denote the tensor size after the second compression as $\alpha M$.
Then the second compression time is $h_1(\alpha M)$ and the communication time for Allgather is $\alpha (n-1)M)$.
The second decompression time after Allgather is $nh_2(\alpha M)$.
Hence, the overall communication time is $(n-1)(1/n+\alpha)M/B$ and the overall compression time is $h_1(M) + nh_2(M/n) + h_1(\alpha M) + nh_2(\alpha M)$.
For quantized tensors, $\alpha=1/n$ so that the overall communication time is $2(n-1)M/B$ and the overall compression time is $h_1(M) + h_1(M/n) + 2nh_2(M/n)$.

We take the first process for sparse tensors and the second process for quantized tensors in Table~\ref{table:comp_comm_overhead}, but the decision tree abstraction covers all of them.

\noindent \textbf{Gather/Broadcast.} 
There are two possible processes for compression with Alltoall/Allgather as the communication.
One is compression, Gather, Broadcast, and decompression.
The compression time is $h_1(M)$.
The communication time for Gather is $\frac{(n-1)M}{B}$.
The tensor size at the root node after Gather is $nM$.
Hence, the communication time for Broadcast is $nM/B$~\cite{broadcast}.
The decompression time is $nh_2(M)$.
The overall communication time is $\frac{(2n-1)M}{B}$ and the overall compression time is $h_1(M) + nh_2(M)$. 

The other process is compression, Gather, decompression, compression, Broadcast, and decompression.
The compression time is $h_1(M)$.
The communication time for Gather is $\frac{(n-1)M}{B}$.
The tensor size at the root node after Gather is $nM$.
The decompression time after Alltoall is $nh_2(M)$.
Similar to Alltoall/Allgather for sparse tensors, the second compression can keep the same compression rate, or change it to another rate.
Without loss of generality, we denote the tensor size after the second compression as $\alpha M$.
Then the second compression time is $h_1(\alpha M)$ and the communication time for Broadcast is $\alpha M/B$.
The second decompression time after Allgather is $h_2(\alpha M)$.
Hence, the overall communication time is $(n-1)M/B + \alpha M/B$ and the overall compression time is $h_1(M) + nh_2(M) + h_1(\alpha M) + h_2(\alpha M)$.
For quantized tensors, $\alpha=1$ so that the overall communication time is $nM/B$ and the overall compression time is $2h_1(M) + (n+1)h_2(M/n)$.

We take the first process for sparse tensors and the second process for quantized tensors in Table~\ref{table:comp_comm_overhead}, but the decision tree abstraction covers all of them.

\section{Valid Connections of Action Tasks}
\label{app:action_tasks}
\begin{figure*}[t!]
\begin{center}
\includegraphics[width=\linewidth]{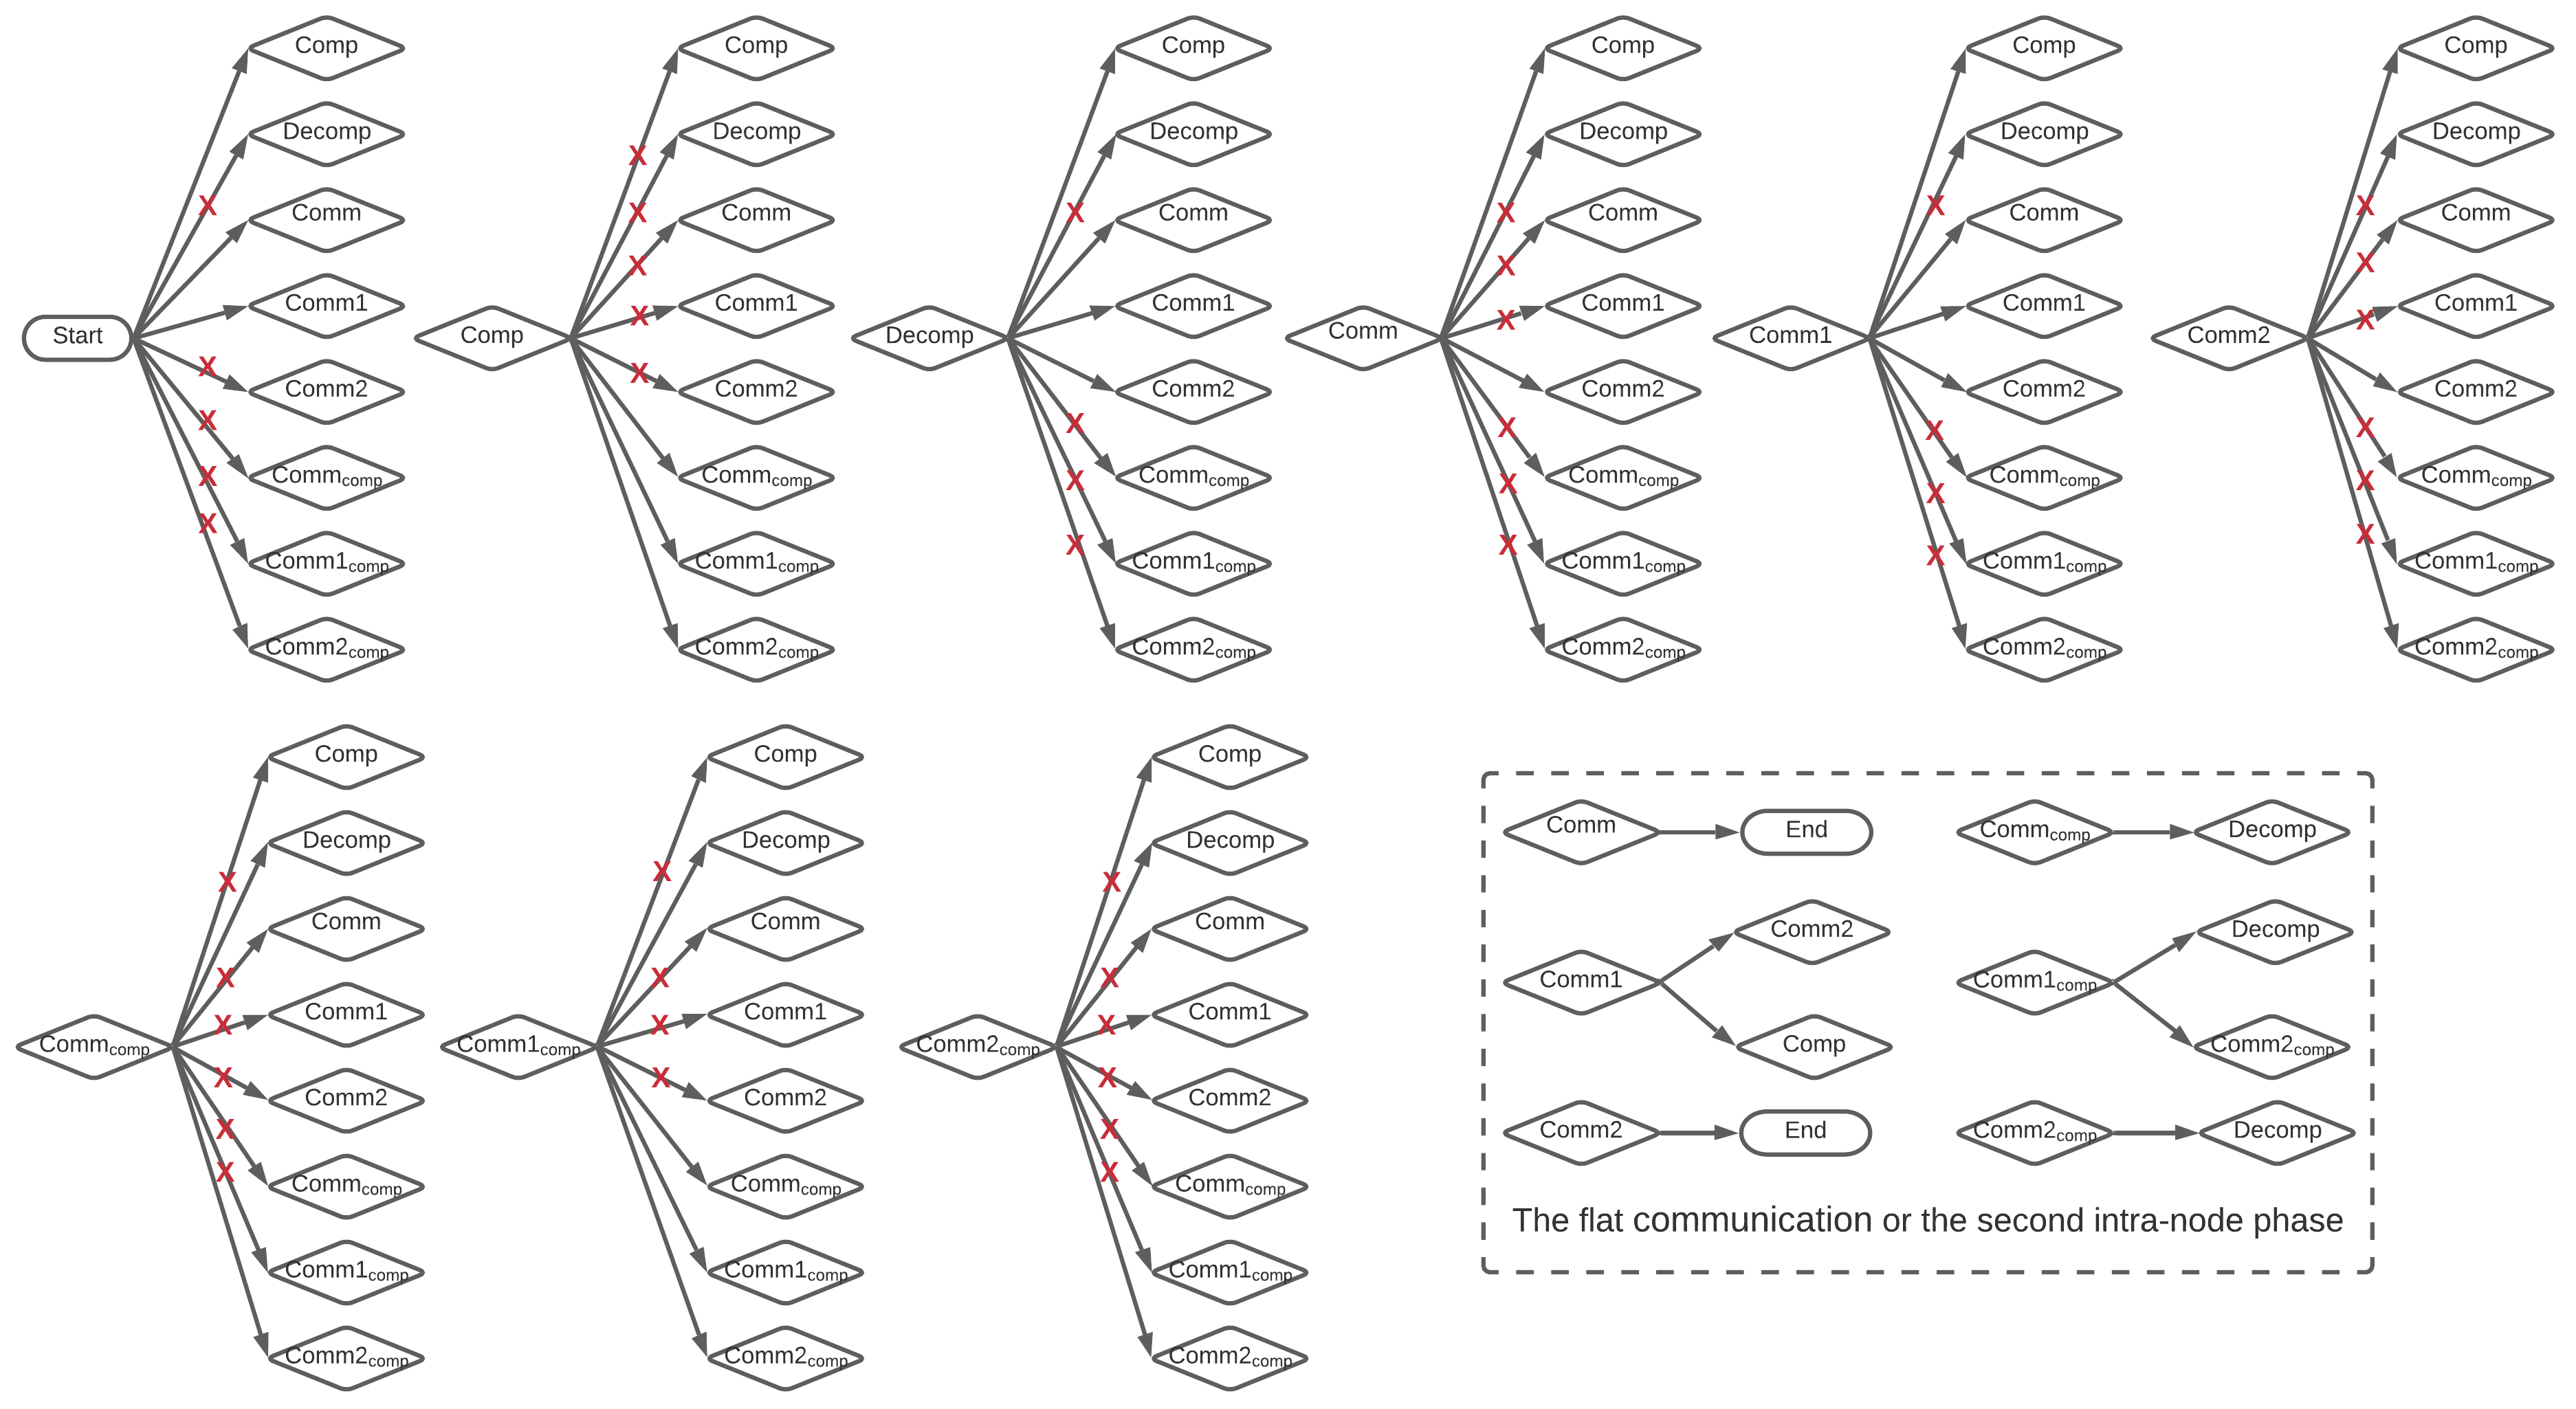}
\vskip -0.1in
\caption{The valid connections of action tasks.}
\label{fig:all_action_tasks}
\end{center}
\end{figure*}

Figure~\ref{fig:all_action_tasks} illustrates the valid connection of all the actions tasks for the decision tree abstraction.
We explain how to prune invalid connection for these tasks.
For convenience, Start of the decision tree is also viewed as an action task.

\noindent \textbf{Start.}
At the beginning, the tensor is uncompressed.
We can rule out Decomp, $Comm_{comp}$, $Comm1_{comp}$, and $Comm2_{comp}$ because they are for compressed tensors.
Comm2 is also pruned because it is not in the correct phase. 
Hence, Comp, Comm and $Comm_1$ are left as the valid connection of Start.

\noindent \textbf{Comp.}
After a tensor is compressed, it cannot be compressed again.
It should not be decompressed intermediately because there is no benefits to compress and decompress a tensor without any communication.
Task Comm, Comm1 and Comm2 are ruled out because they are communication tasks for uncompressed data.
Therefore, $Comm_{comp}$, $Comm1_{comp}$, and $Comm2_{comp}$ are left as the valid connections of Task Comp.

\noindent \textbf{Decomp.}
After a tensor is decompressed, it cannot be decompressed again.
The tensor becomes uncompressed data so that $Comm_{comp}$, $Comm1_{comp}$, and $Comm2_{comp}$ are ruled out.
Therefore, Comp, Comm, Comm1, and Comm2 are left as the valid connections of Task Decomp.

\noindent \textbf{Comm.}
After Comm, the tensor is still uncompressed data so that Decomp, $Comm_{comp}$, $Comm1_{comp}$, and $Comm2_{comp}$ are ruled out.
In flat communication, there is no other communication tasks after Comm;
in hierarchical communication, Comm is only valid as the indivisible routine for inter-node communication.
Therefore, Comm and Comm1 are also invalid as the connection of Comm.
Only Comp and Comm2 are left as the valid connections of Task Comm. 

\noindent \textbf{Comm1.}
After Comm1, the tensor is still uncompressed data so that Decomp, $Comm_{comp}$, $Comm1_{comp}$, and $Comm2_{comp}$ are ruled out.
All the other action tasks are valid connections of Task Comm1.

\noindent \textbf{Comm2.}
After Comm2, the tensor is still uncompressed data so that Decomp, $Comm_{comp}$, $Comm1_{comp}$, and $Comm2_{comp}$ are ruled out.
In flat communication, there is no other communication tasks after Comm2;
in hierarchical communication, Comm2 is only valid for the second inter-node communication phase or the second intra-node communication phase. 
Therefore, Comm and Comm1 are also invalid as the connection of Comm2.
Only Comp and Comm2 are left as the valid connections of Task Comm2.

\noindent \textbf{Comm}$_{comp}$.
After $Comm_{comp}$, the tensor is compressed data so that Comp, Comm, Comm1, Comm2 are ruled out.
In flat communication, there is no other communication tasks after $Comm_{comp}$;
in hierarchical communication, $Comm_{comp}$ is only valid as the indivisible routine for inter-node communication. 
Therefore, $Comm_{comp}$ and $Comm1_{comp}$ are also invalid as the connection of Comm2.
Only Decomp and $Comm2_{comp}$ are left as the valid connections of Task $Comm_{comp}$.

\noindent \textbf{Comm1}$_{comp}$.
After $Comm1_{comp}$, the tensor is compressed data so that Comp, Comm, Comm1, Comm2 are ruled out.
All the other action tasks are valid connections of Task $Comm1_{comp}$.

\noindent \textbf{Comm2}$_{comp}$.
After $Comm2_{comp}$, the tensor is compressed data so that Comp, Comm, Comm1, Comm2 are ruled out.
In flat communication, there is no other communication tasks after $Comm2_{comp}$;
in hierarchical communication, $Comm2_{comp}$ is only valid for the second inter-node communication phase or the second intra-node communication phase. 
Therefore, $Comm_{comp}$ and $Comm1_{comp}$ are also invalid as the connection of Comm2.
Only Comp and $Comm2_{comp}$ are left as the valid connections of Task $Comm2_{comp}$.

We observe that the valid connections of communication tasks can be further pruned in flat communication or in the second intra-node phase.
For example, there is no other decision tasks after Comm and Comm2.
The only valid task after $Comm_{comp}$ and $Comm2_{comp}$ is Decomp.
In flat communication, Comm1 has two valid connections: Comm2 and Comp; $Comm1_{comp}$ also has two valid connections: Decomp and $Comm2_{comp}$.
These special cases are illustrated at the dotted box in Figure~\ref{fig:all_action_tasks}.

At the beginning of synchronization, {\name} needs to determine flat or hierarchical communication. 
Hence, the only \textit{flat comm?} appears right after Start.
% \footnote{Start and End are dummy tasks to describe compression options.}
\textit{compress?} appears for uncompressed tensors as long as they need communications.
\textit{divisible scheme?} appears once in each communication pattern.
In flat communication, it appears before any communication tasks; in hierarchical communication, it appears before inter-machine communication.

There are three \textit{pruning rules} to construct the tree.
The first rule is that the following action tasks of an action task must be its valid connections.
The second rule is that the communication tasks must match the correct steps.
For example, Comm1 and Comm1$_{comp}$ are only valid as the first steps of divisible schemes.
Task Comm2 and $Comm2_{comp}$ is only valid as the second step of a divisible scheme, 
Comm and $Comm_{comp}$ are only valid as the indivisible schemes.
The third rule is that the choices of communication tasks in the first and second steps must match.
For example, if Comm1 is Alltoall, Comm2 in this divisible scheme must be Allgather.
Each path from Start to End is a valid compression option.

\begin{figure*}[ht!]
    \centering
    \begin{subfigure}[t]{0.24\linewidth}
	\includegraphics[width=\linewidth]{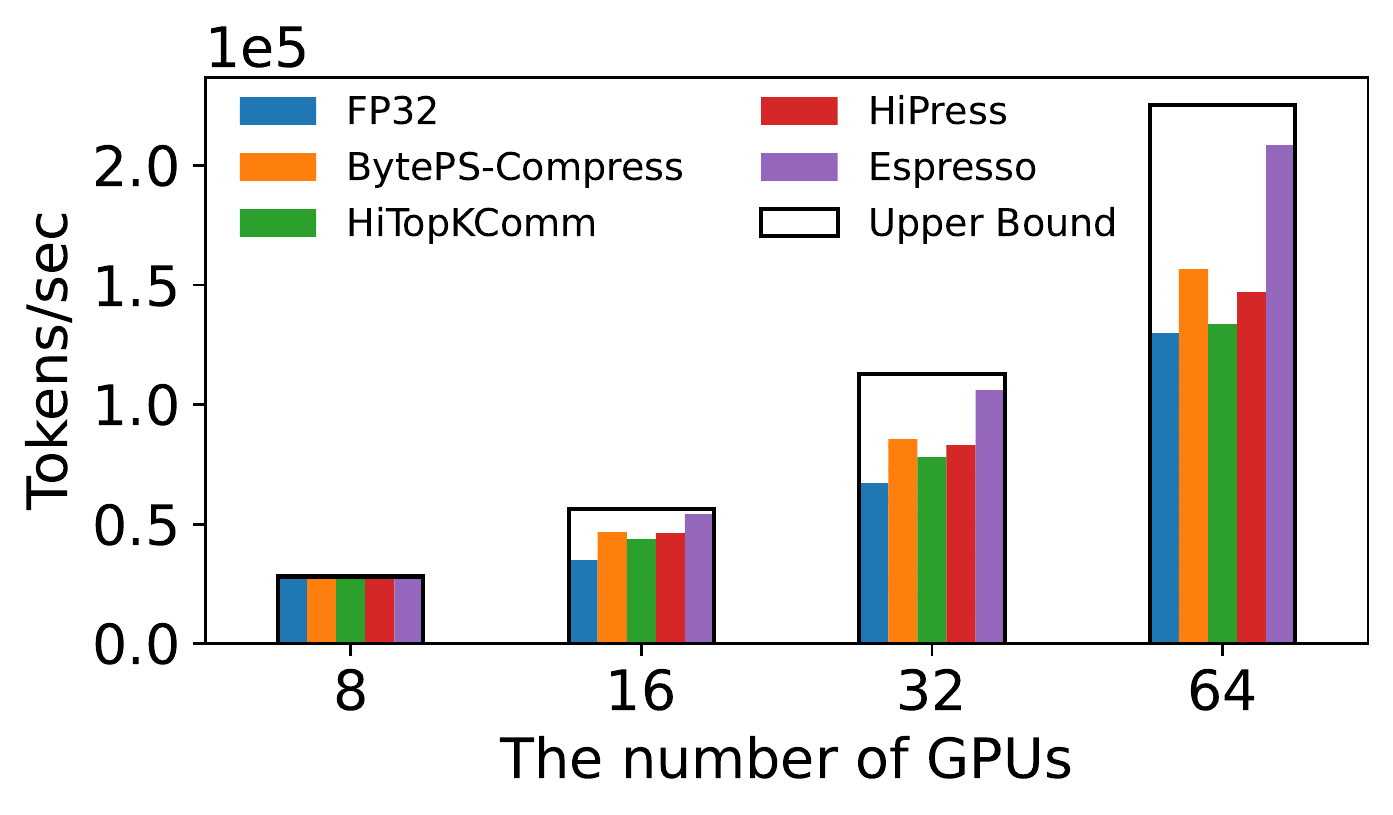}
	\vskip -0.1in
	\caption{BERT + Randomk}
    \end{subfigure}    
	\begin{subfigure}[t]{0.24\linewidth}
	\includegraphics[width=\linewidth]{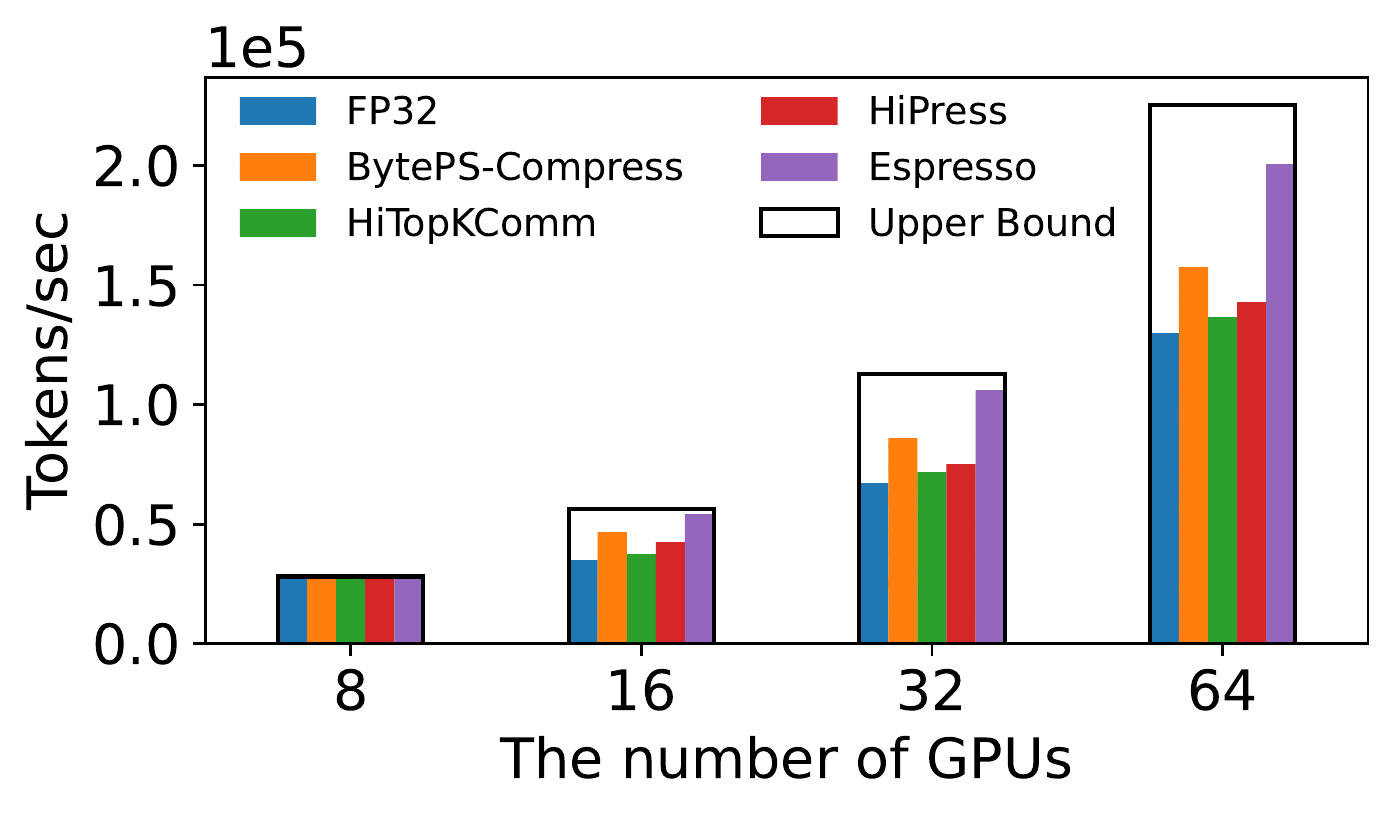}
	\vskip -0.1in
	\caption{BERT + DGC}
    \end{subfigure}  
    \begin{subfigure}[t]{0.24\linewidth}
	\includegraphics[width=\linewidth]{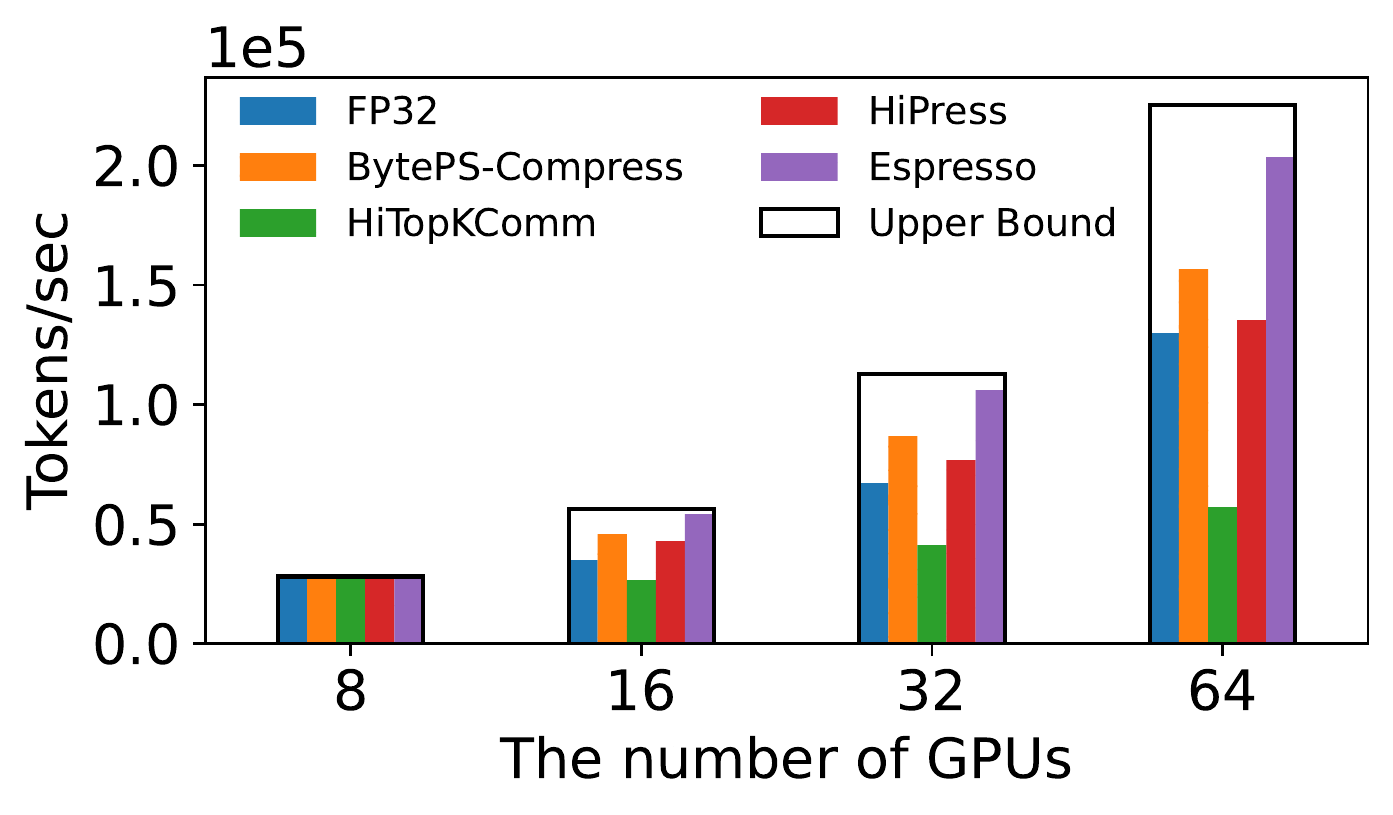}
	\vskip -0.1in
	\caption{BERT + EFSignSGD}
    \end{subfigure}  
    \begin{subfigure}[t]{0.24\linewidth}
	\includegraphics[width=\linewidth]{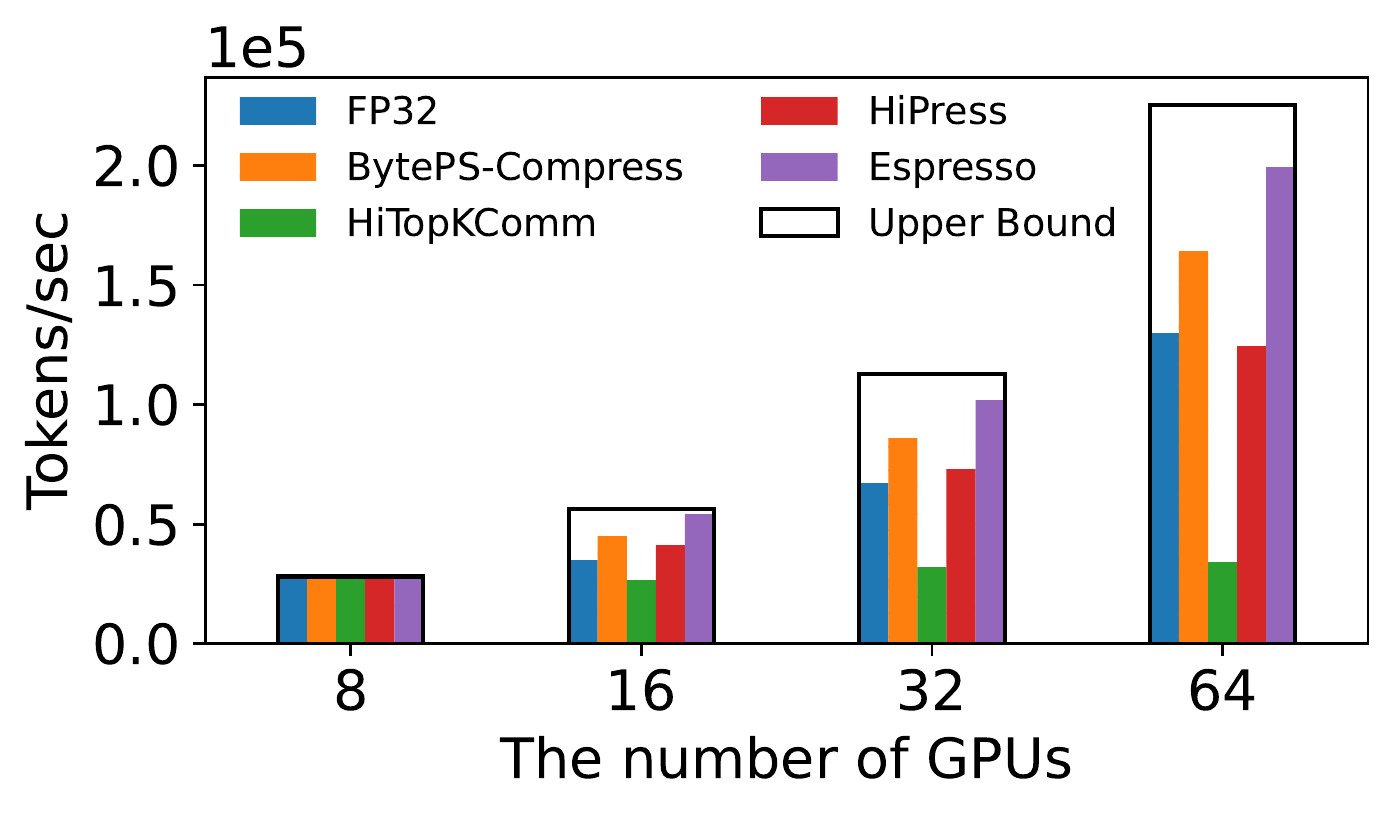}
	\vskip -0.1in
	\caption{BERT + Onebit}
    \end{subfigure}  
    \vskip -0.1in
    \caption{The training throughput of BERT with NVLink-based GPU machines and 100Gbps network.}
    \label{fig:nvlink_bert}
\end{figure*}

\begin{figure*}[h!]
    \centering
    \begin{subfigure}[t]{0.24\linewidth}
	\includegraphics[width=\linewidth]{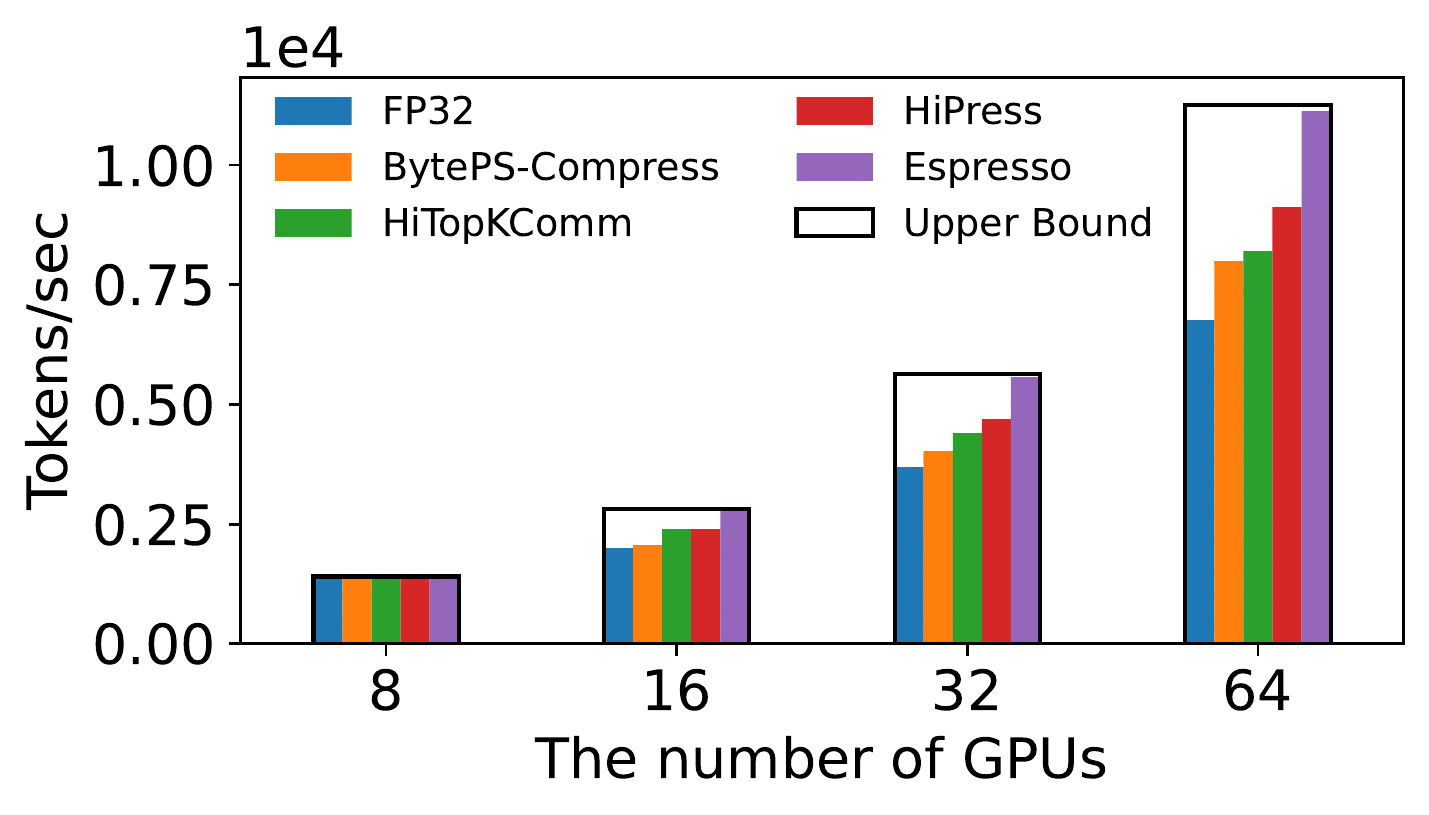}
	\vskip -0.1in
	\caption{GPT2 + Randomk}
    \end{subfigure}    
	\begin{subfigure}[t]{0.24\linewidth}
	\includegraphics[width=\linewidth]{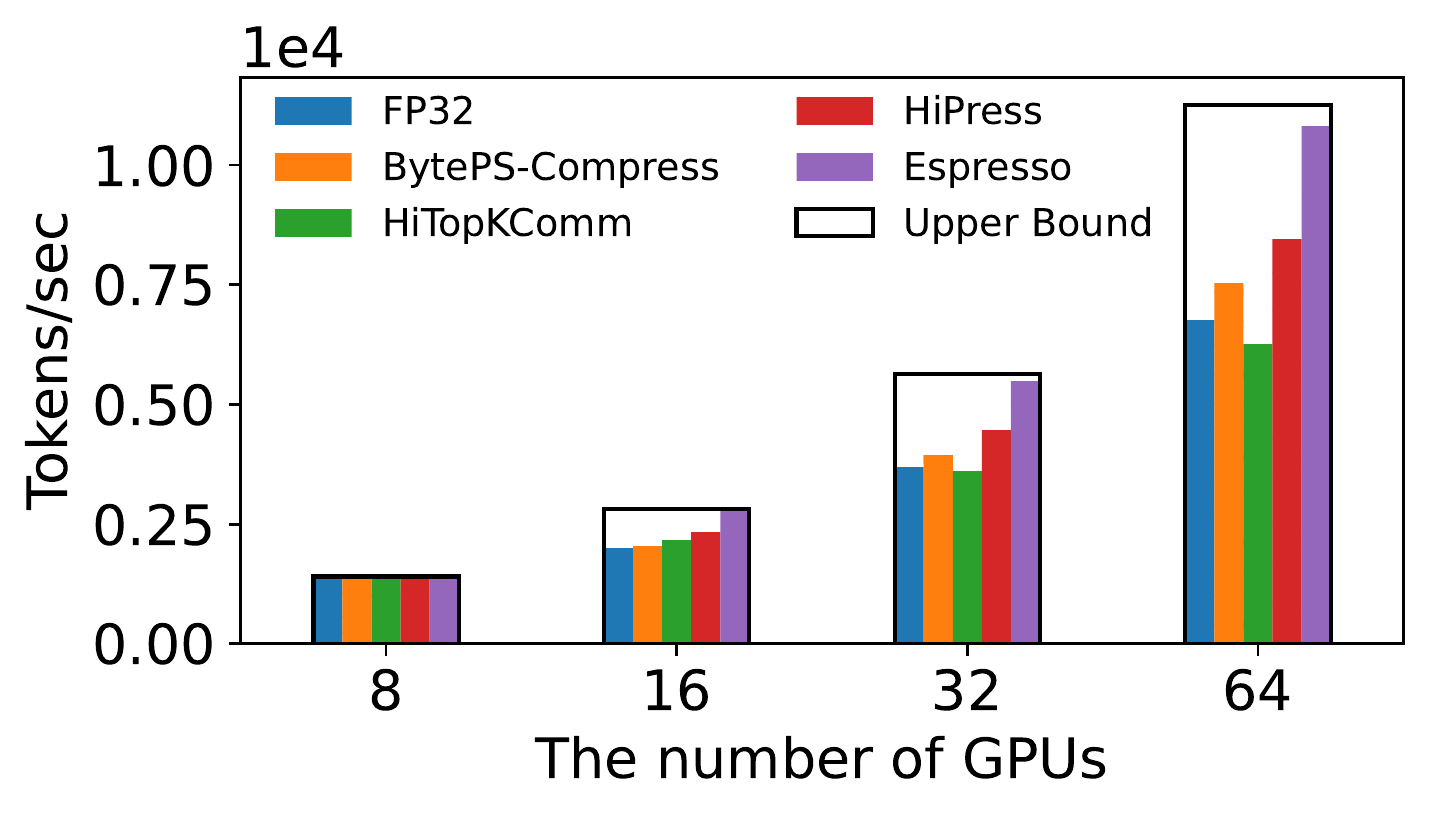}
	\vskip -0.1in
	\caption{GPT2 + DGC}
    \end{subfigure}  
    \begin{subfigure}[t]{0.24\linewidth}
	\includegraphics[width=\linewidth]{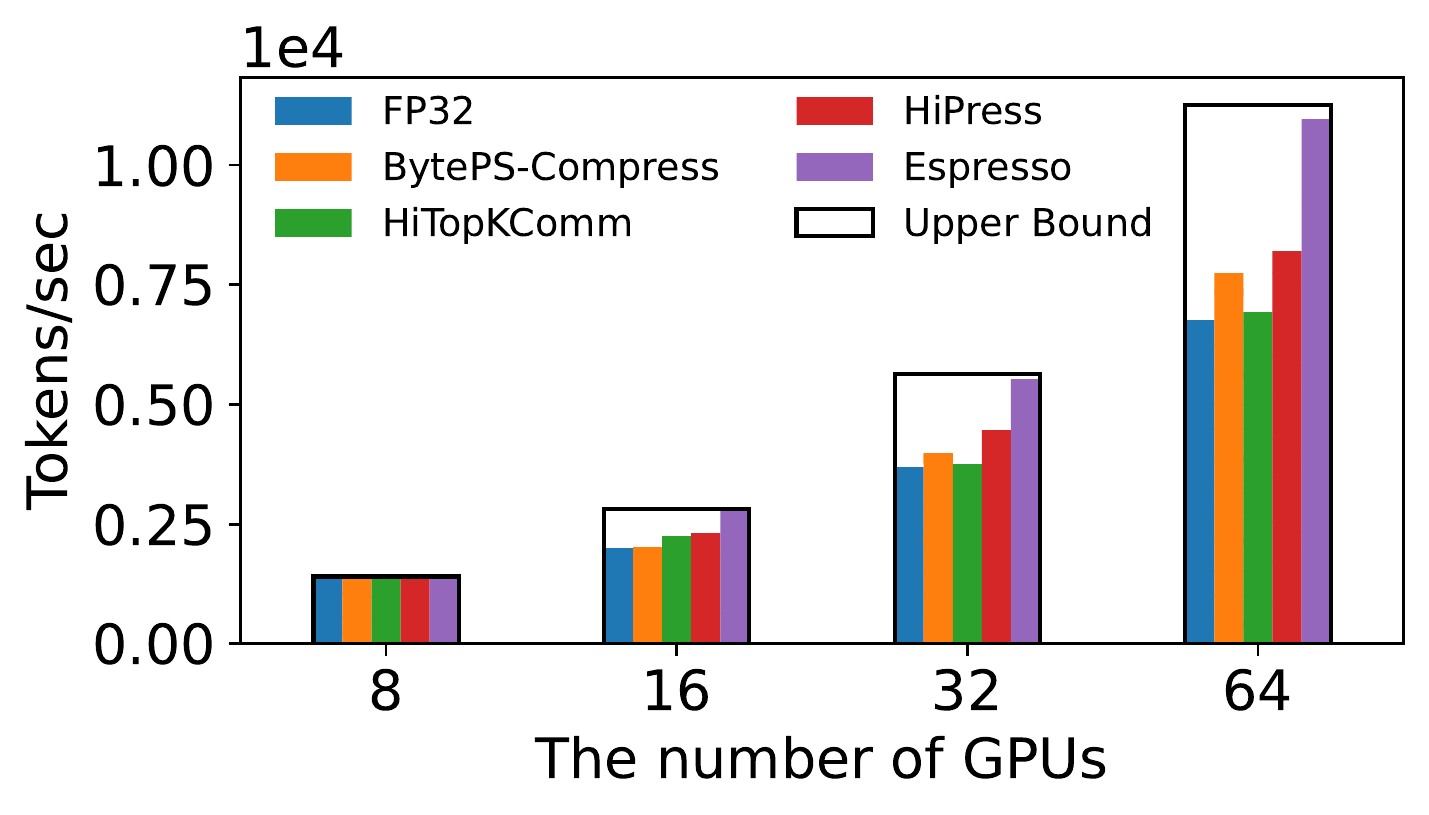}
	\vskip -0.1in
	\caption{GPT2 + EFSignSGD}
    \end{subfigure}  
    \begin{subfigure}[t]{0.24\linewidth}
	\includegraphics[width=\linewidth]{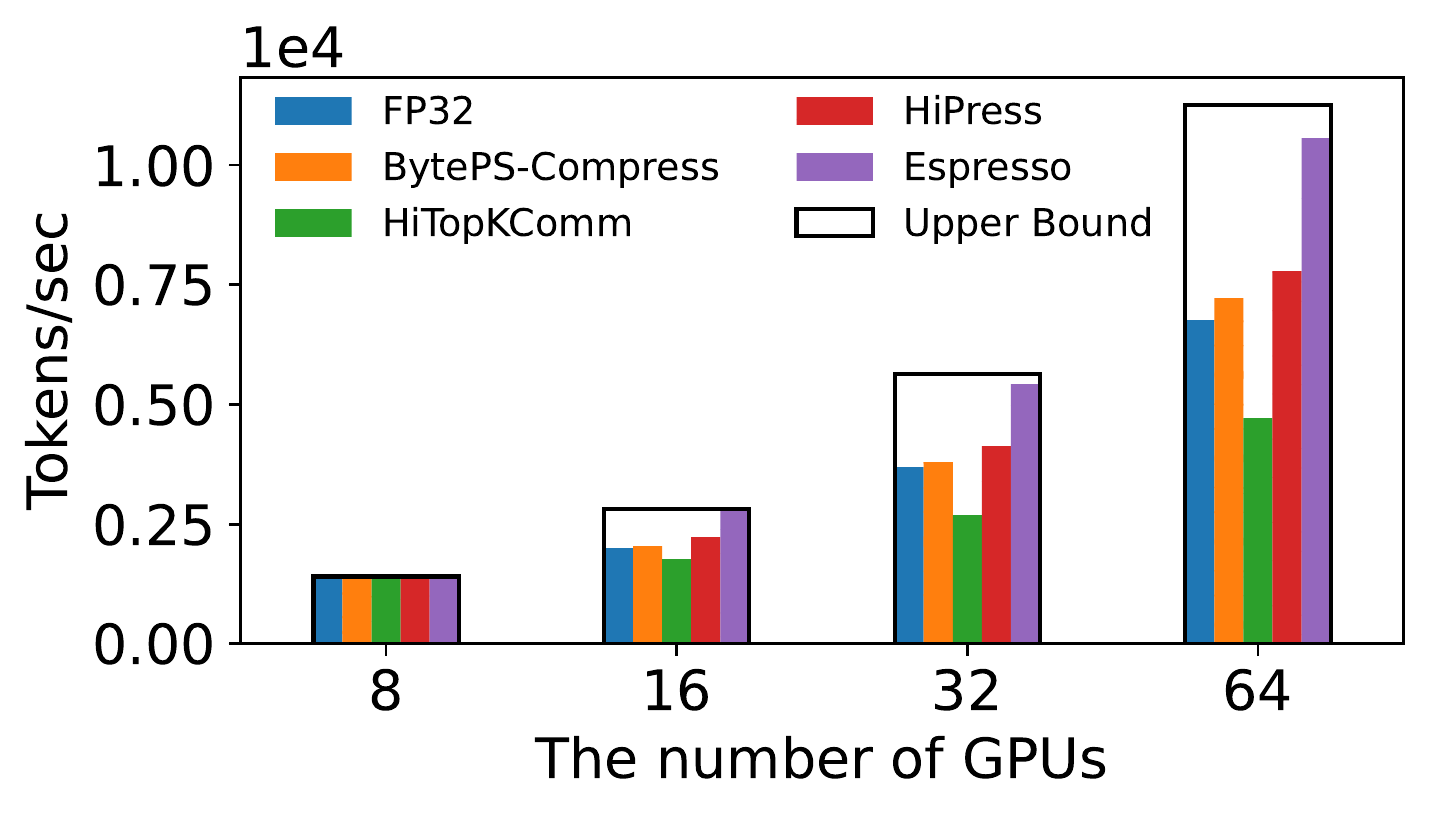}
	\vskip -0.1in
	\caption{GPT2 + Onebit}
    \end{subfigure}  
    \vskip -0.1in
    \caption{The training throughput of GPT2 with NVLink-based GPU machines and 100Gbps network.}
    \label{fig:nvlink_gpt2}
\end{figure*}

\begin{figure*}[h]
    \centering
    \begin{subfigure}[t]{0.24\linewidth}
	\includegraphics[width=\linewidth]{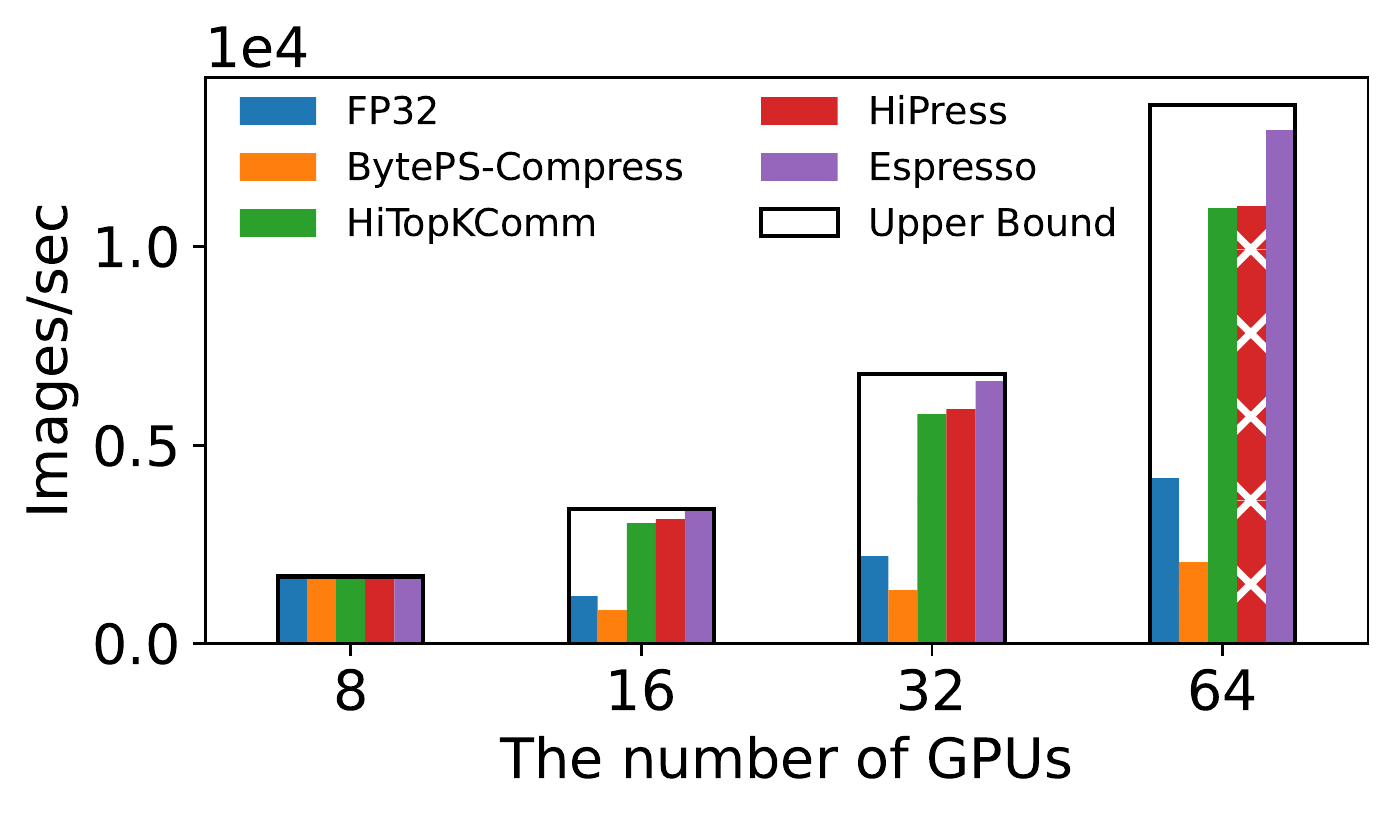}
	\vskip -0.1in
	\caption{VGG16 + Randomk}
    \end{subfigure}    
	\begin{subfigure}[t]{0.24\linewidth}
	\includegraphics[width=\linewidth]{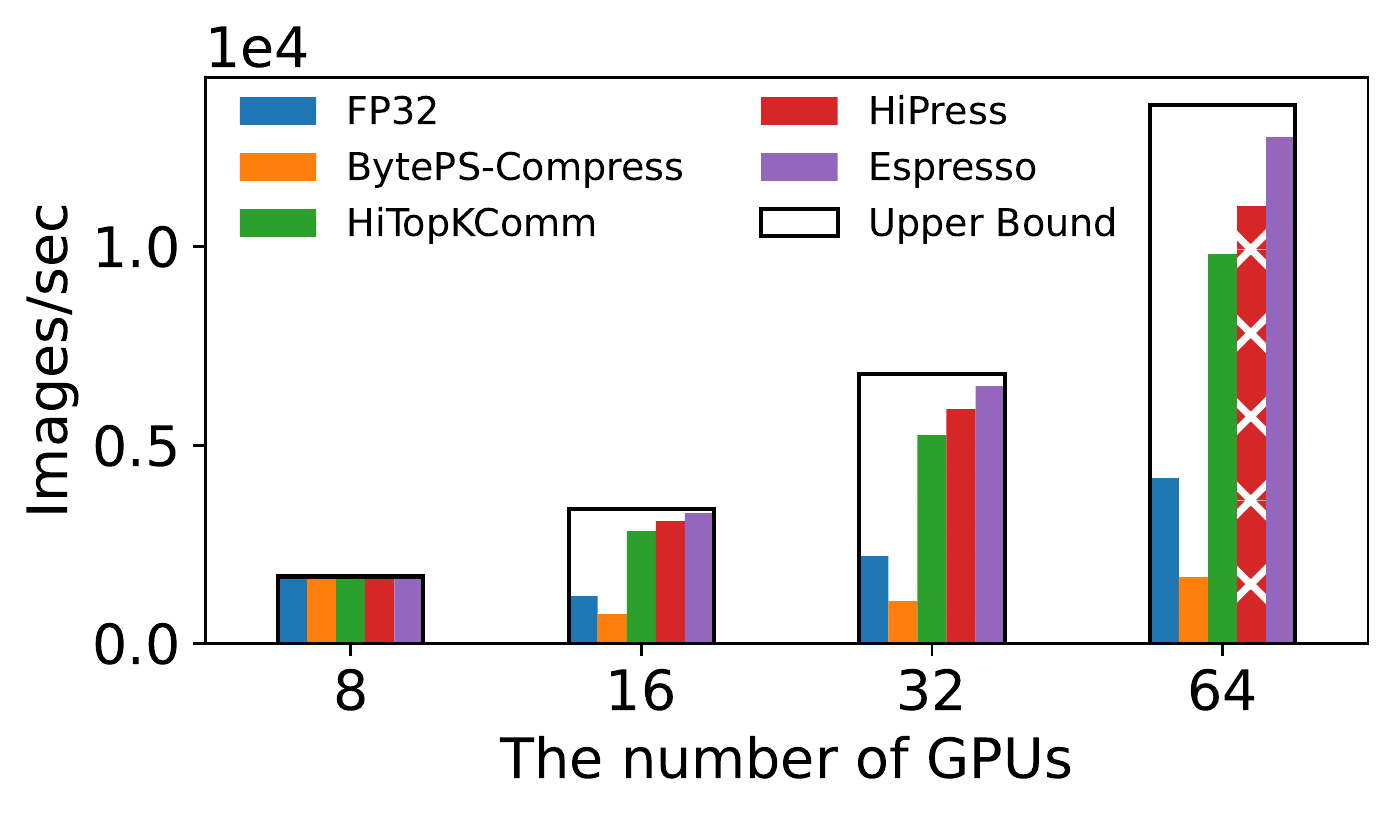}
	\vskip -0.1in
	\caption{VGG16 + DGC}
    \end{subfigure}  
    \begin{subfigure}[t]{0.24\linewidth}
	\includegraphics[width=\linewidth]{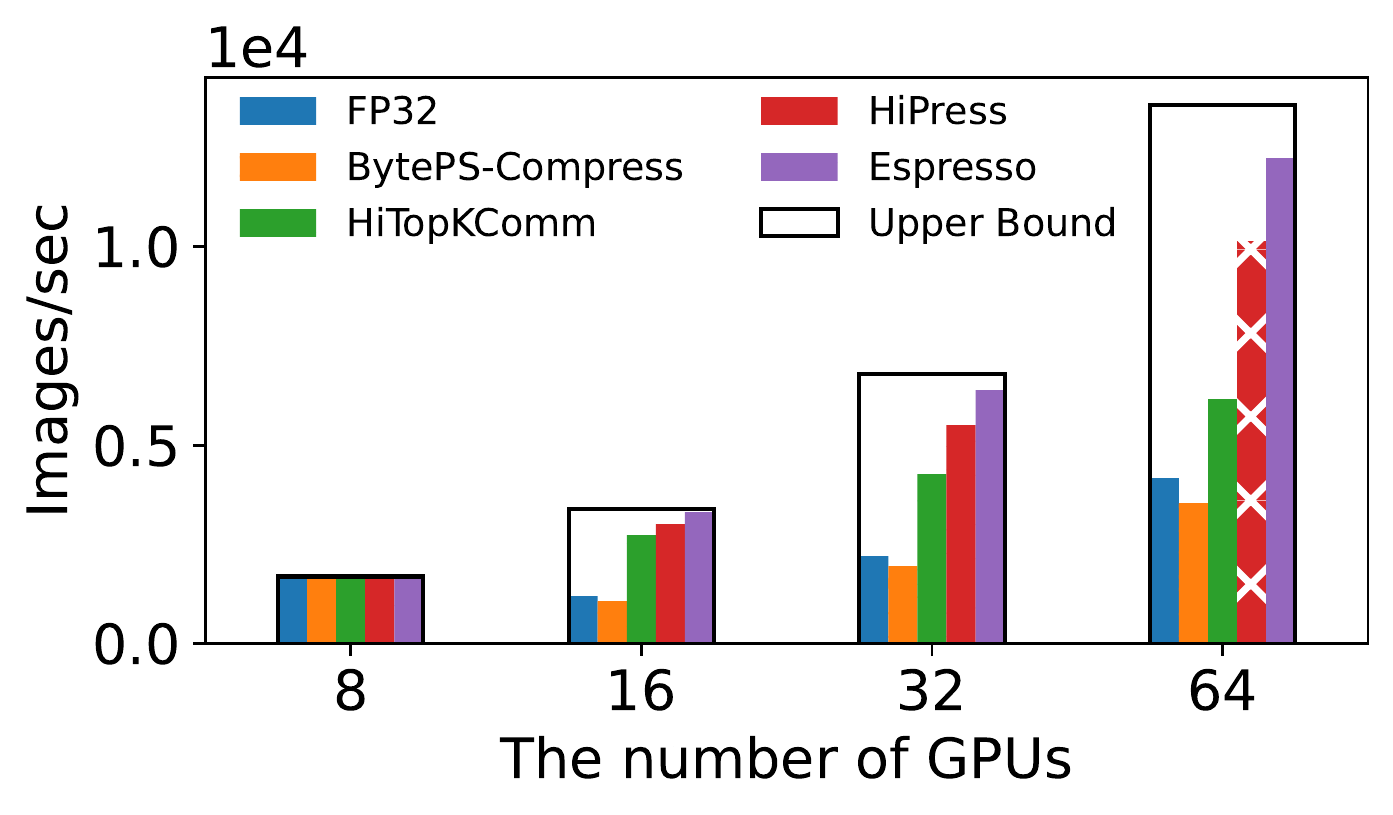}
	\vskip -0.1in
	\caption{VGG16 + EFSignSGD}
    \end{subfigure}  
    \begin{subfigure}[t]{0.24\linewidth}
	\includegraphics[width=\linewidth]{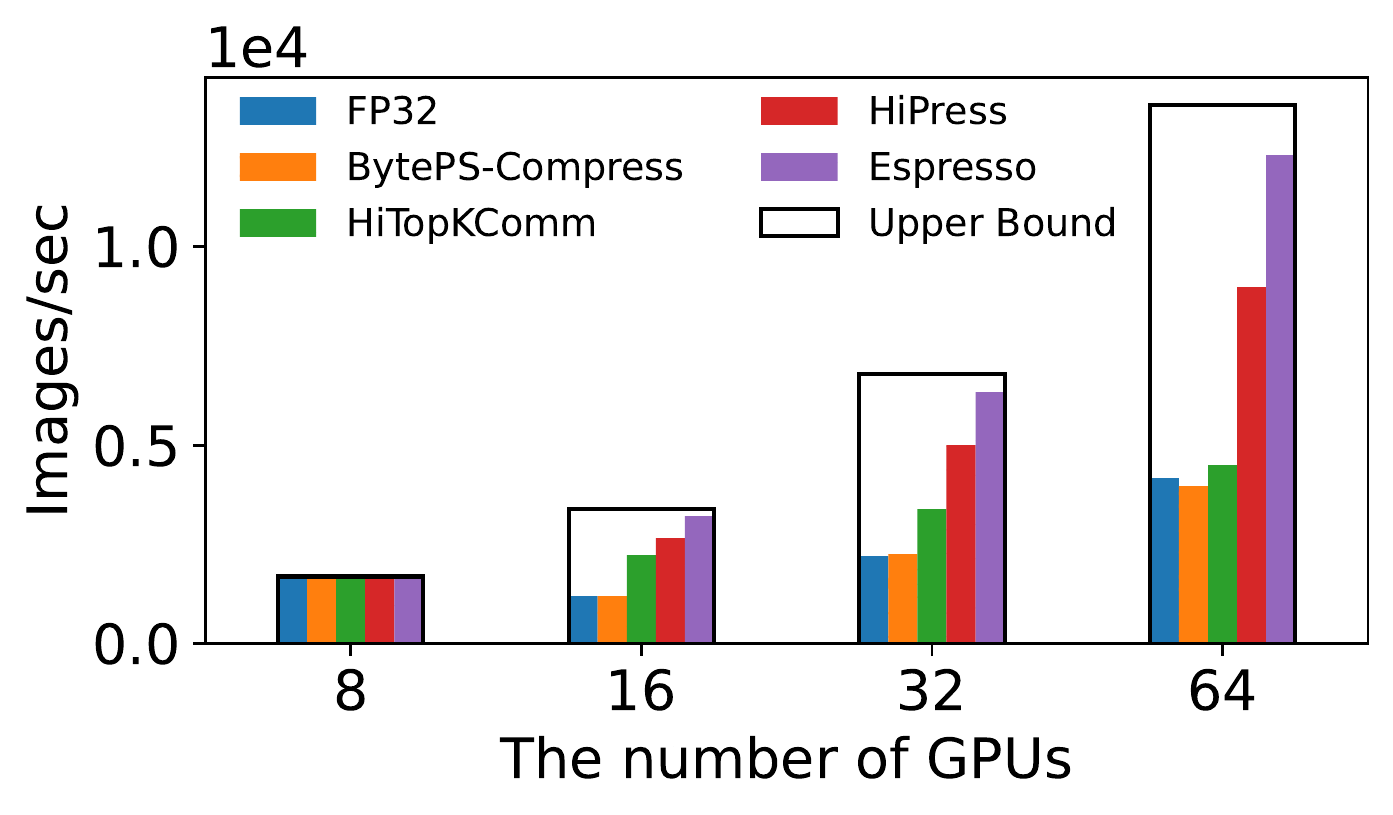}
	\vskip -0.1in
	\caption{VGG16 + Onebit}
    \end{subfigure}  
    \vskip -0.1in
    \caption{The training throughput of VGG16 with NVLink-based GPU machines and 100Gbps network.}
    \label{fig:nvlink_vgg16}
\end{figure*}

\begin{figure*}[h]
    \centering
    \begin{subfigure}[t]{0.24\linewidth}
	\includegraphics[width=\linewidth]{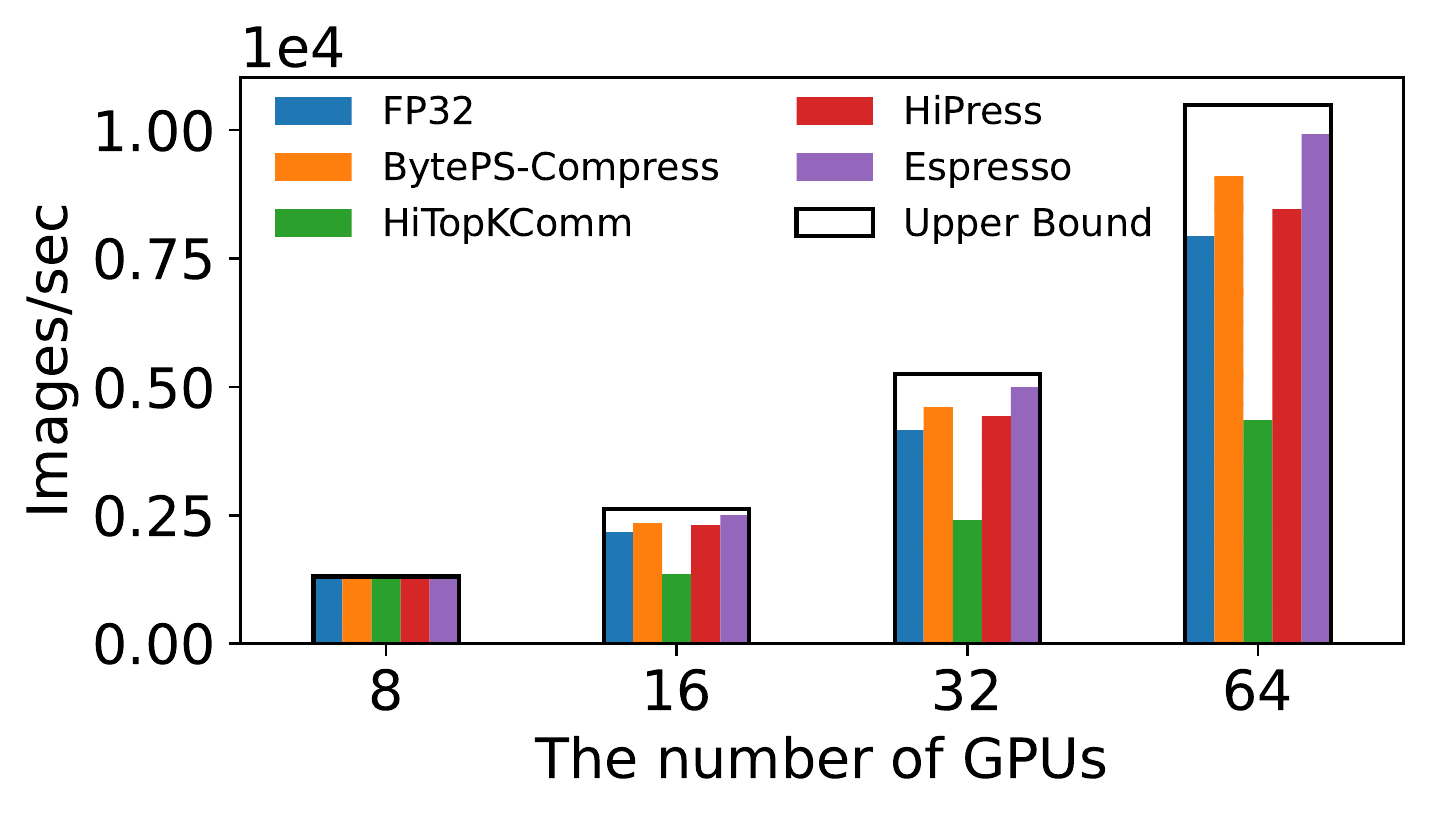}
	\vskip -0.1in
	\caption{ResNet101 + Randomk}
    \end{subfigure}    
	\begin{subfigure}[t]{0.24\linewidth}
	\includegraphics[width=\linewidth]{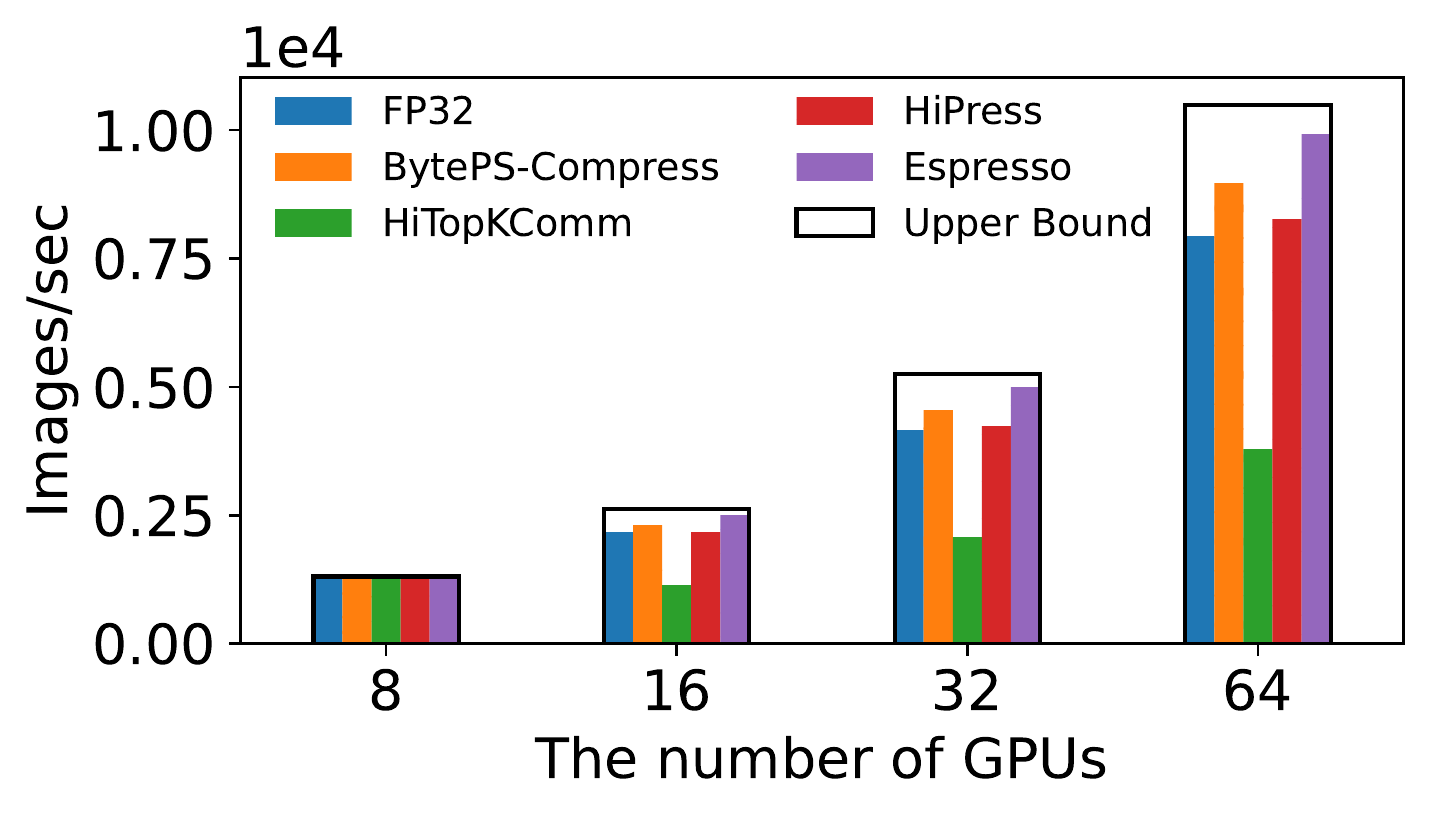}
	\vskip -0.1in
	\caption{ResNet101 + DGC}
    \end{subfigure}  
    \begin{subfigure}[t]{0.24\linewidth}
	\includegraphics[width=\linewidth]{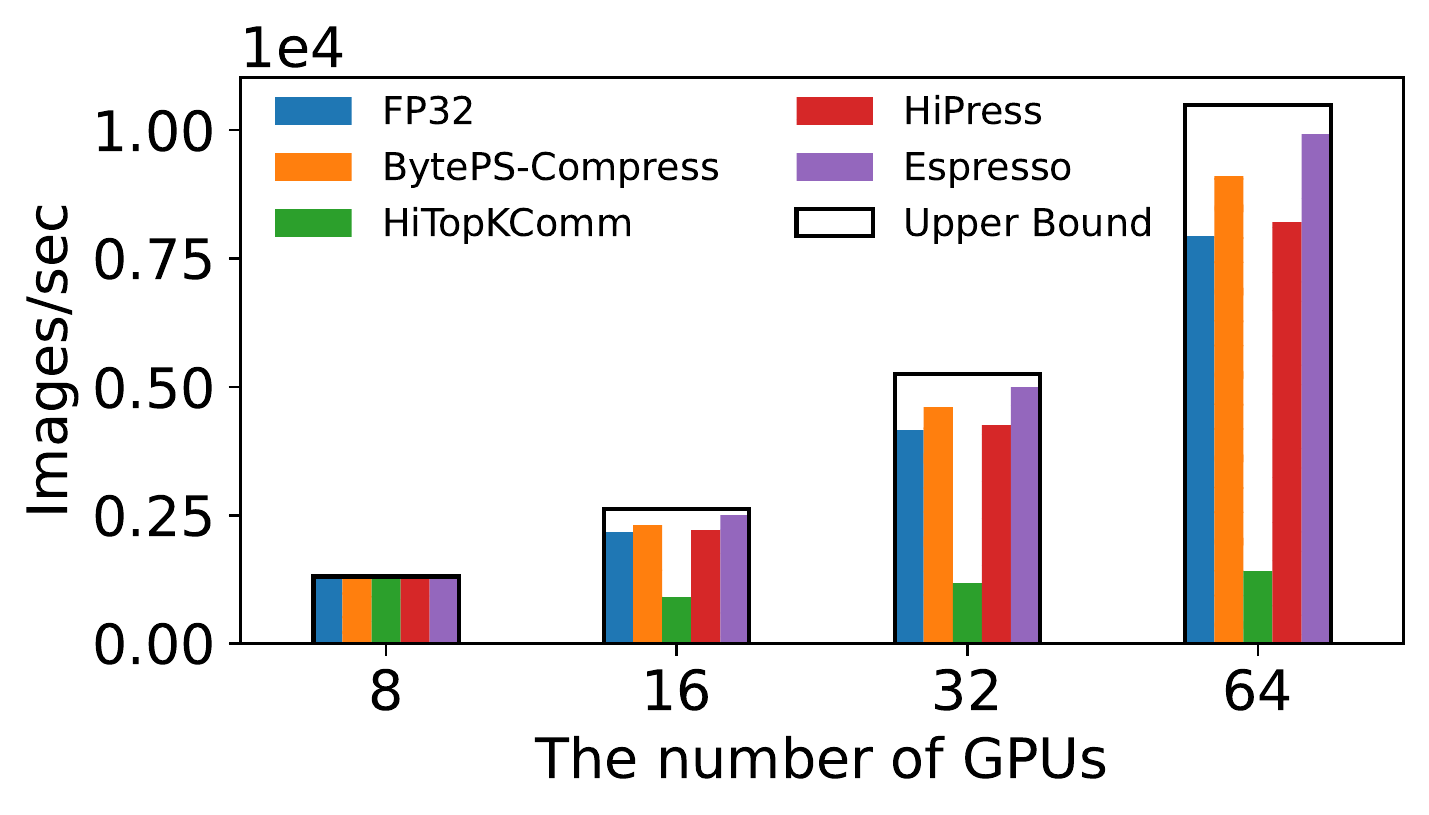}
	\vskip -0.1in
	\caption{ResNet101 + EFSignSGD}
    \end{subfigure}  
    \begin{subfigure}[t]{0.24\linewidth}
	\includegraphics[width=\linewidth]{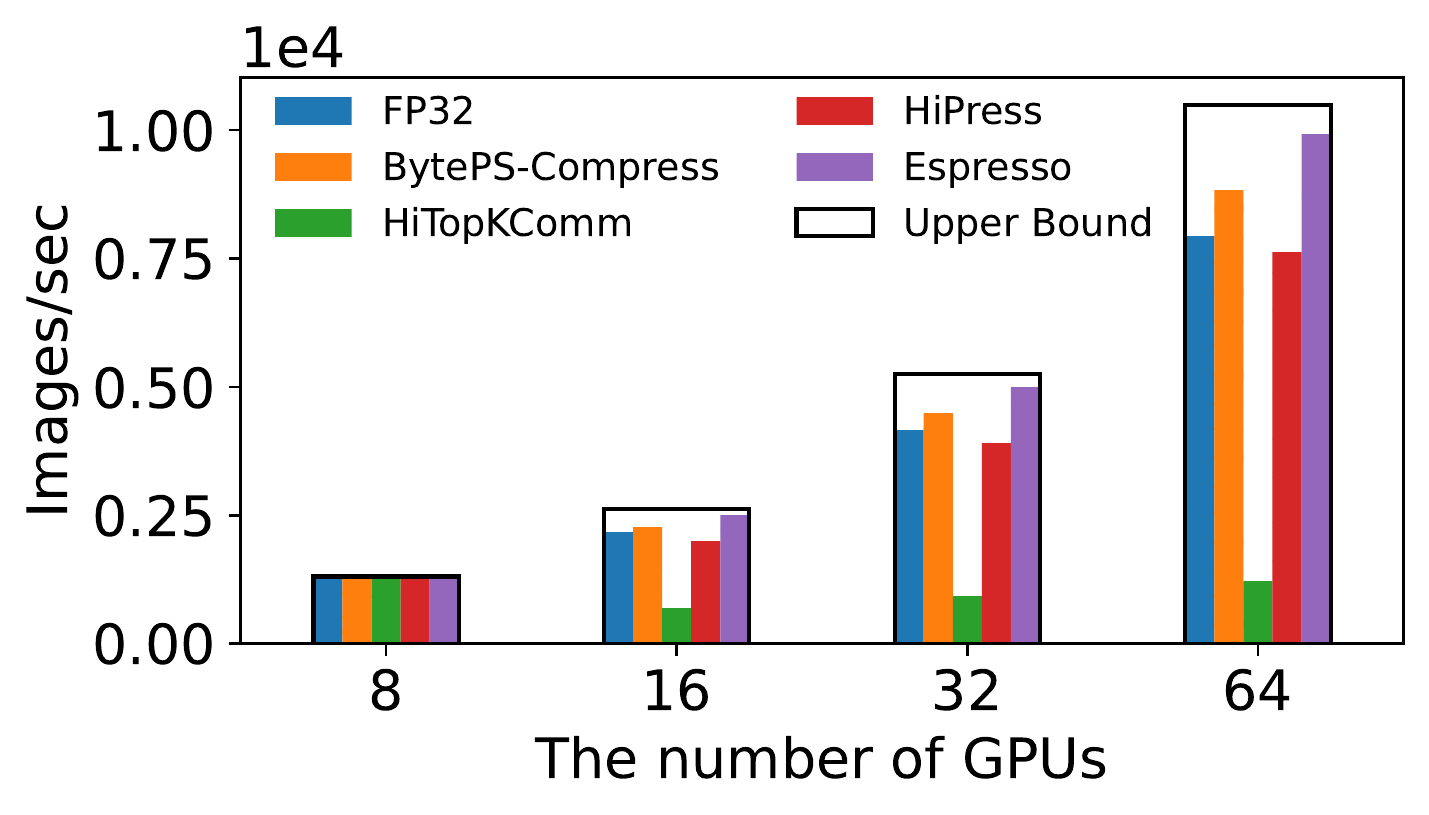}
	\vskip -0.1in
	\caption{ResNet101 + Onebit}
    \end{subfigure}  
    \vskip -0.1in
    \caption{The training throughput of ResNet101 with NVLink-based GPU machines and 100Gbps network.}
    \label{fig:nvlink_resnet101}
    \vskip -0.15in
\end{figure*}

\begin{figure*}[h]
    \centering
    \begin{subfigure}[t]{0.24\linewidth}
	\includegraphics[width=\linewidth]{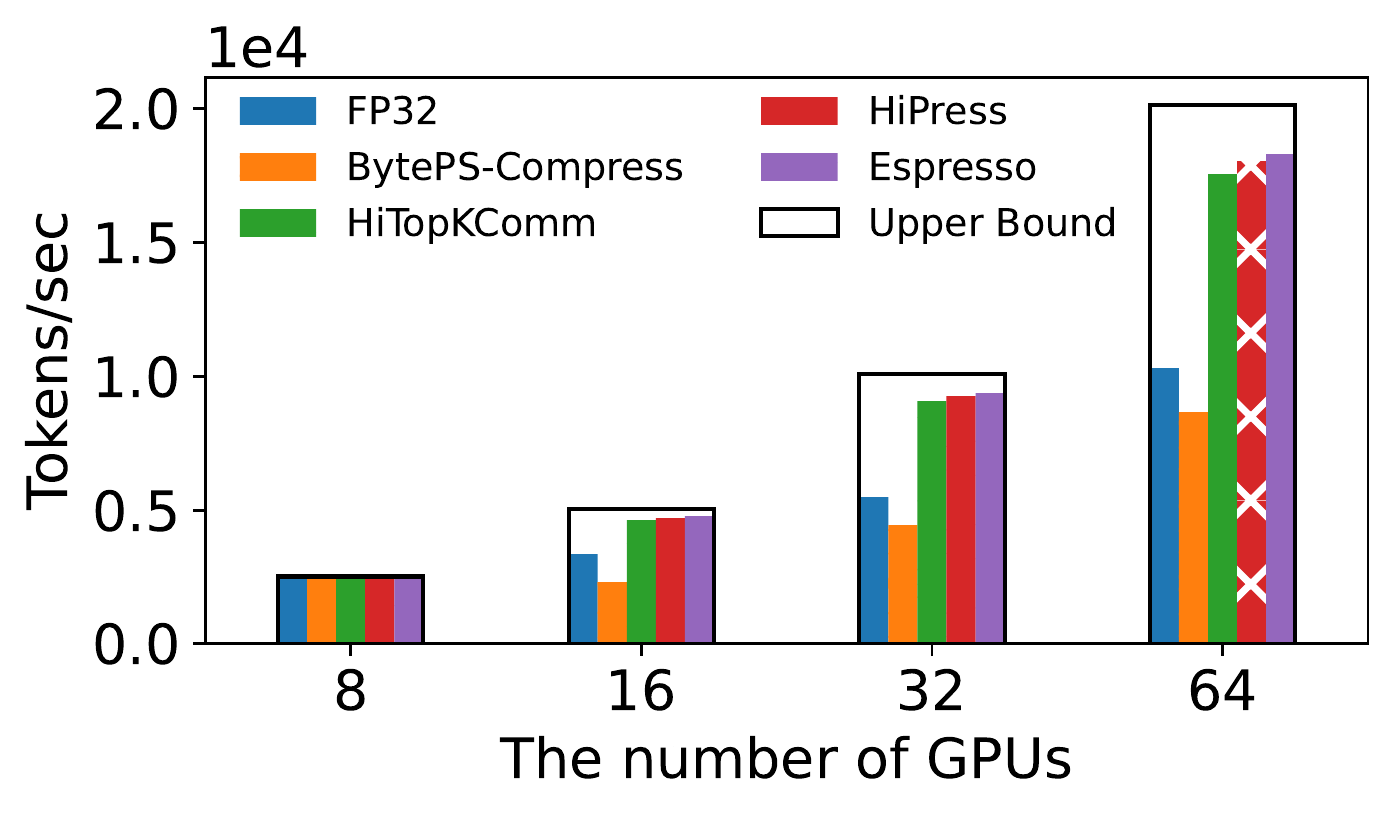}
	\vskip -0.1in
	\caption{LSTM + Randomk}
    \end{subfigure}    
	\begin{subfigure}[t]{0.24\linewidth}
	\includegraphics[width=\linewidth]{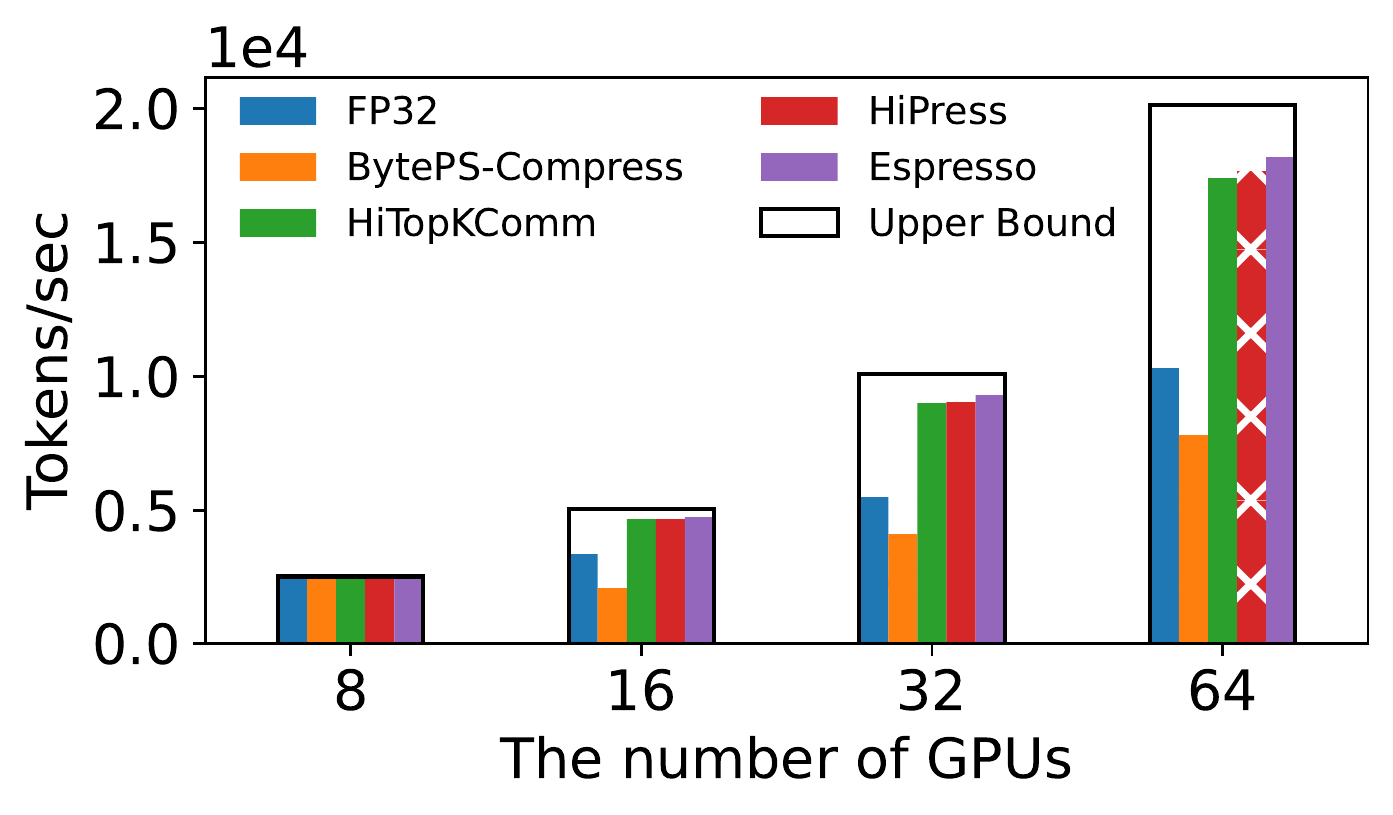}
	\vskip -0.1in
	\caption{LSTM + DGC}
    \end{subfigure}  
    \begin{subfigure}[t]{0.24\linewidth}
	\includegraphics[width=\linewidth]{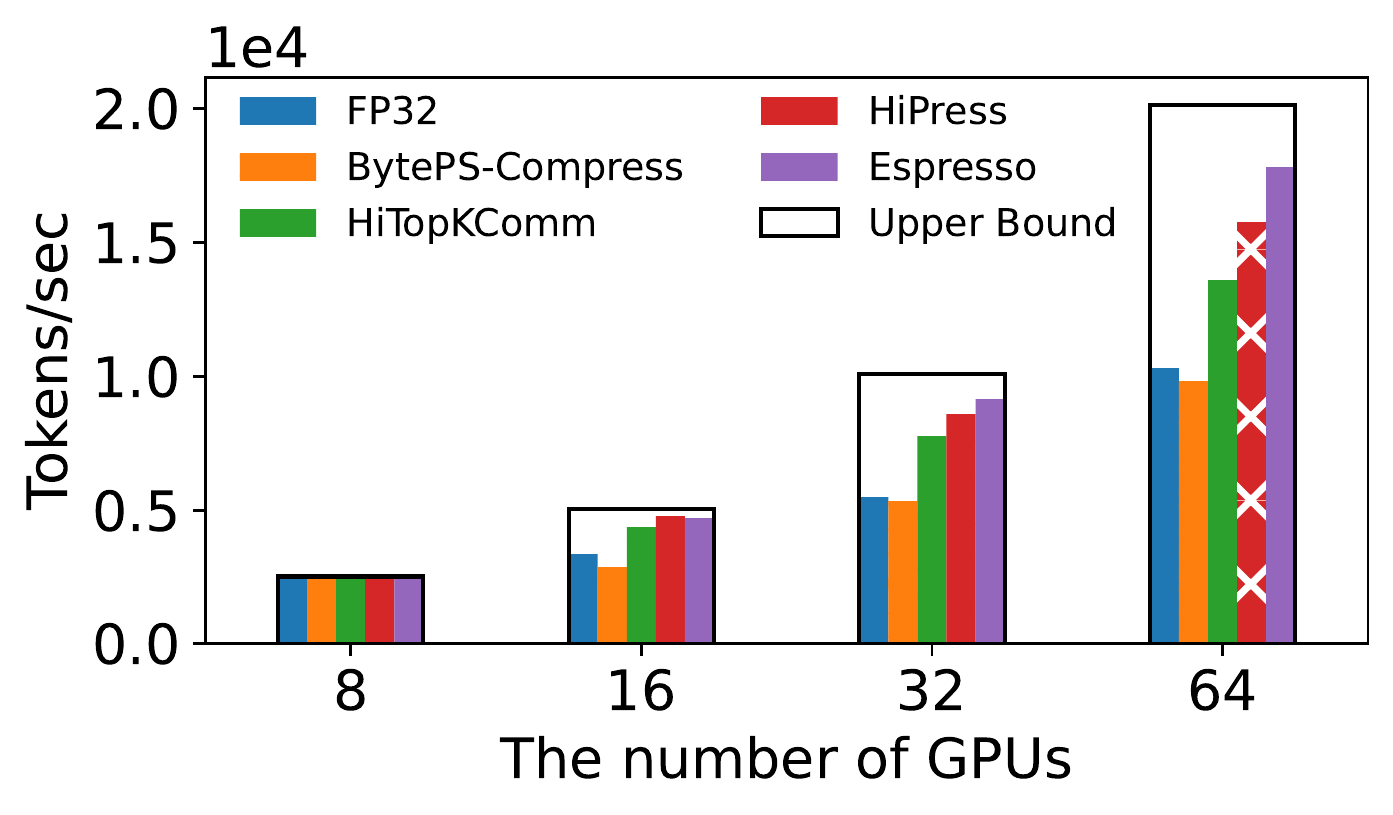}
	\vskip -0.1in
	\caption{LSTM + EFSignSGD}
    \end{subfigure}  
    \begin{subfigure}[t]{0.24\linewidth}
	\includegraphics[width=\linewidth]{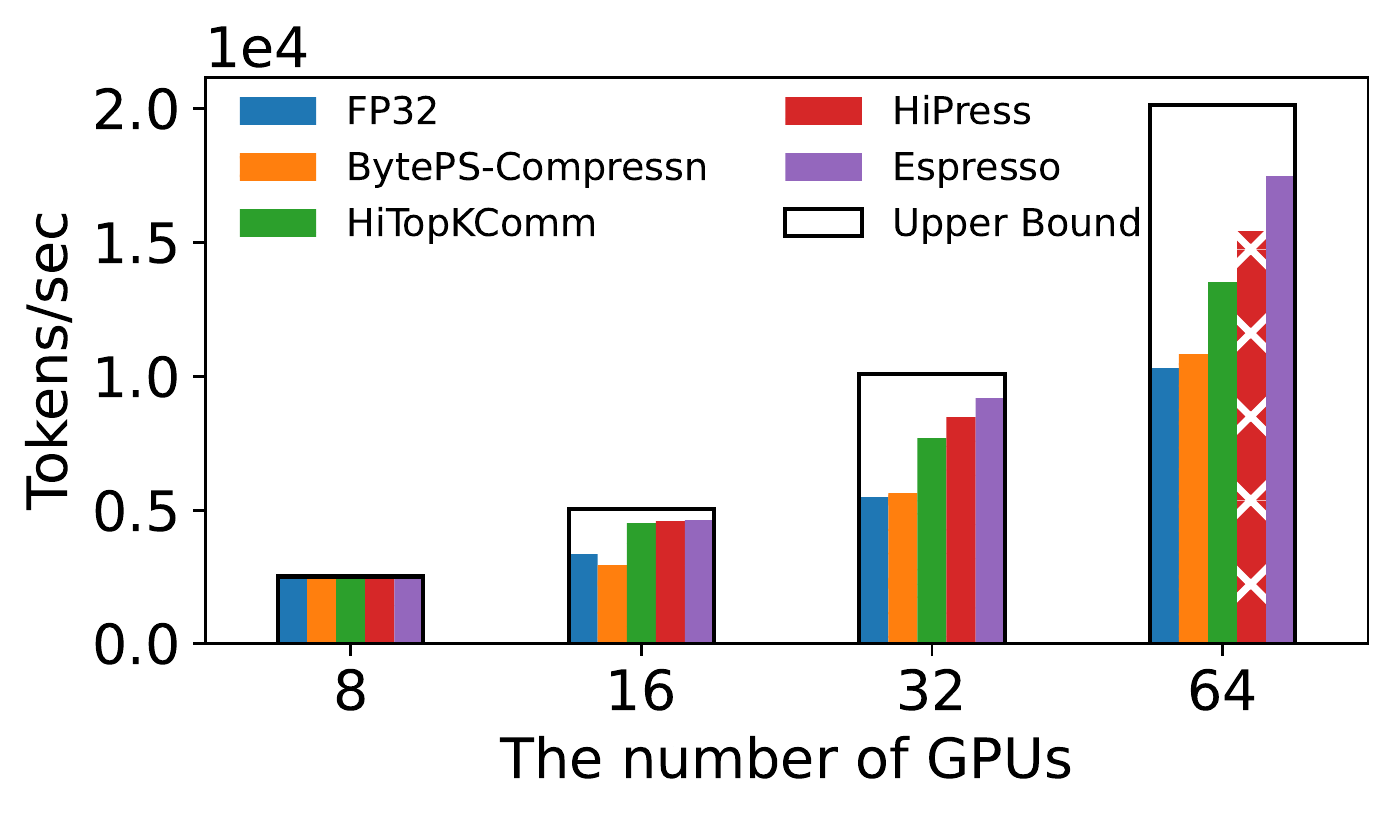}
	\vskip -0.1in
	\caption{LSTM + Onebit}
    \end{subfigure}  
    \vskip -0.1in
    \caption{The training throughput of LSTM with NVLink-based GPU machines and 100Gbps network.}
    \label{fig:nvlink_lstm}
\end{figure*}

\section{Proof of Lemma~\ref{lemma:cpu} and Theorem~\ref{the:cpu}}
\label{app:prove}
\begin{customlemma}{1}
     Suppose $G_i^{gpu}$ needs to offload $q$ tensors to CPUs for compression. The best solution is to offload the first $q$ tensors.
\end{customlemma}

\begin{proof}
    Compression with GPUs or CPUs results in the same compressed tensor size and thus the same communication time.
    No matter which $q$ tensors are selected for CPU offloading, they incur the same GPU compression time and have the same amount of delay on computation.
    They also lead to the same CPU compression time.
    The difference between different offloading solutions lies in the overlapping time between the CPU compression time and the communication time.
    
    $G_q = \{B_{g_1}, B_{g_2}, \cdots, B_{g_q}\}$ is set of the first $q$ tensors in $G_i^{gpu}$. 
    We take a different set $G'_q = \{B_{g_1'}, B_{g_2'}, \cdots, B_{g_q'}\}$ with $q$ tensors and the tensors are sorted in descending order of their distances to the output layer.
    The first difference in the two sets is $g_i \ne g_i'$.
    Because $B_{g_i}$ appears earlier than $B_{g_i'}$, the CPU compression and the corresponding communication of this tensor can start no later than before.
    Replacing $B_{g_i'}$ with $B_{g_i}$ in $G'_q$ can increase the overlapping time, or at least not make it worse.
    We can always replace tensors in $G'_q $ in this way until it becomes $G_q$.
    Therefore, $G_q$ is the best set of tensors for CPU offloading.
\end{proof}

\begin{customthm}{1}
    {\name} can find the best CPU offloading solution in $O(\prod (|G_i^{gpu}|+1))$.
\end{customthm}

\begin{proof}
We first prove that given a $U = \{u_1, u_2, \cdots, u_d\}$, the best CPU offloading is to offload the first $u_i$ tensors in $G_i^{gpu}$ to CPUs.
Without loss of generality, we assume that in the best CPU offloading, the $u_j$ offloaded tensors in $G_j^{gpu}$ are not the first $u_j$ tensors, which contradicts the conclusion in Lemma~\ref{lemma:cpu}.
Then the assumption does not hold.

Because the number of tensors in $G_i^{gpu}$ is $|G_i^{gpu}|$, there are $|G_i^{gpu}| + 1$ options for the number of tensors for CPU offloading, from $0$ tensors to $|G_i^{gpu}|$ tensors.
Therefore, the number of possible $U$ in $\mathcal{U}$ is $O(\prod (|G_i^{gpu}|+1))$.
For each $U$, its best offloading solution is determined. 
Therefore, {\name} only needs to traverse the $\prod (|G_i^{gpu}|+1)$ possibilities to find the best CPU offloading.
\end{proof}

\section{Additional Experiments}
\label{app:exp}
\subsection{DDL with NVLink-based GPU Machines}

Figures~\ref{fig:nvlink_bert}-\ref{fig:nvlink_lstm} show the training throughput of BERT-base, GPT2, VGG16, ResNet101, and LSTM with the four GC algorithms, respectively, on NVLink-based GPU Machines.
The network bandwidth is 100Gbps.
These results are consistent with the results shown in Figure~\ref{fig:v100_nvlink}.

\subsection{DDL with PCIe-only GPU Machines}

Figures~\ref{fig:pcie_bert}-\ref{fig:pcie_lstm} show the training throughput of BERT-base, GPT2, VGG16, ResNet101, and LSTM with the four GC algorithms, respectively, on PCIe-only GPU Machines.
The network bandwidth is 25Gbps.
These results are consistent with the results shown in Figure~\ref{fig:v100_pcie}.

\begin{figure*}[h!]
    \centering
    \begin{subfigure}[t]{0.24\linewidth}
	\includegraphics[width=\linewidth]{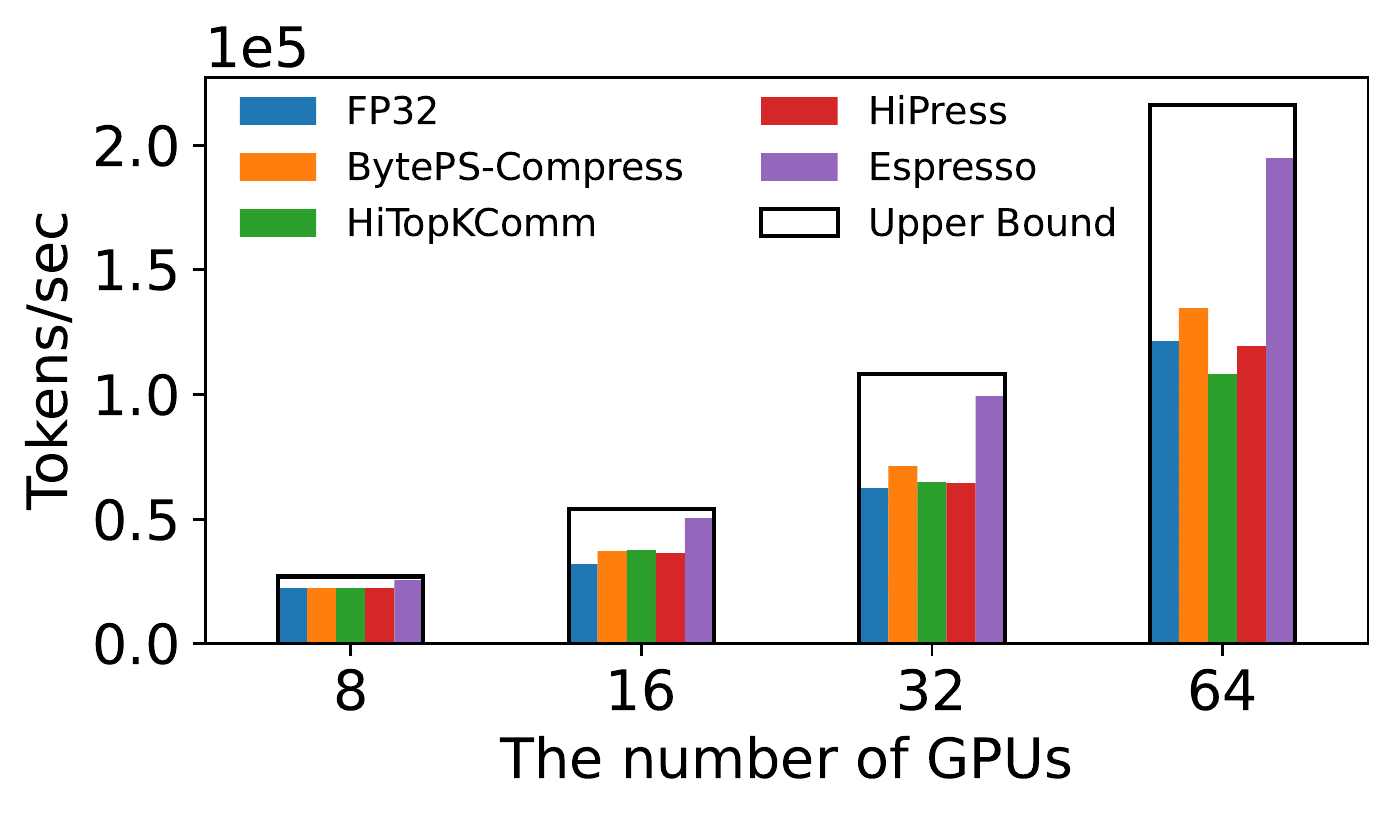}
	\vskip -0.1in
	\caption{BERT + Randomk}
    \end{subfigure}    
	\begin{subfigure}[t]{0.24\linewidth}
	\includegraphics[width=\linewidth]{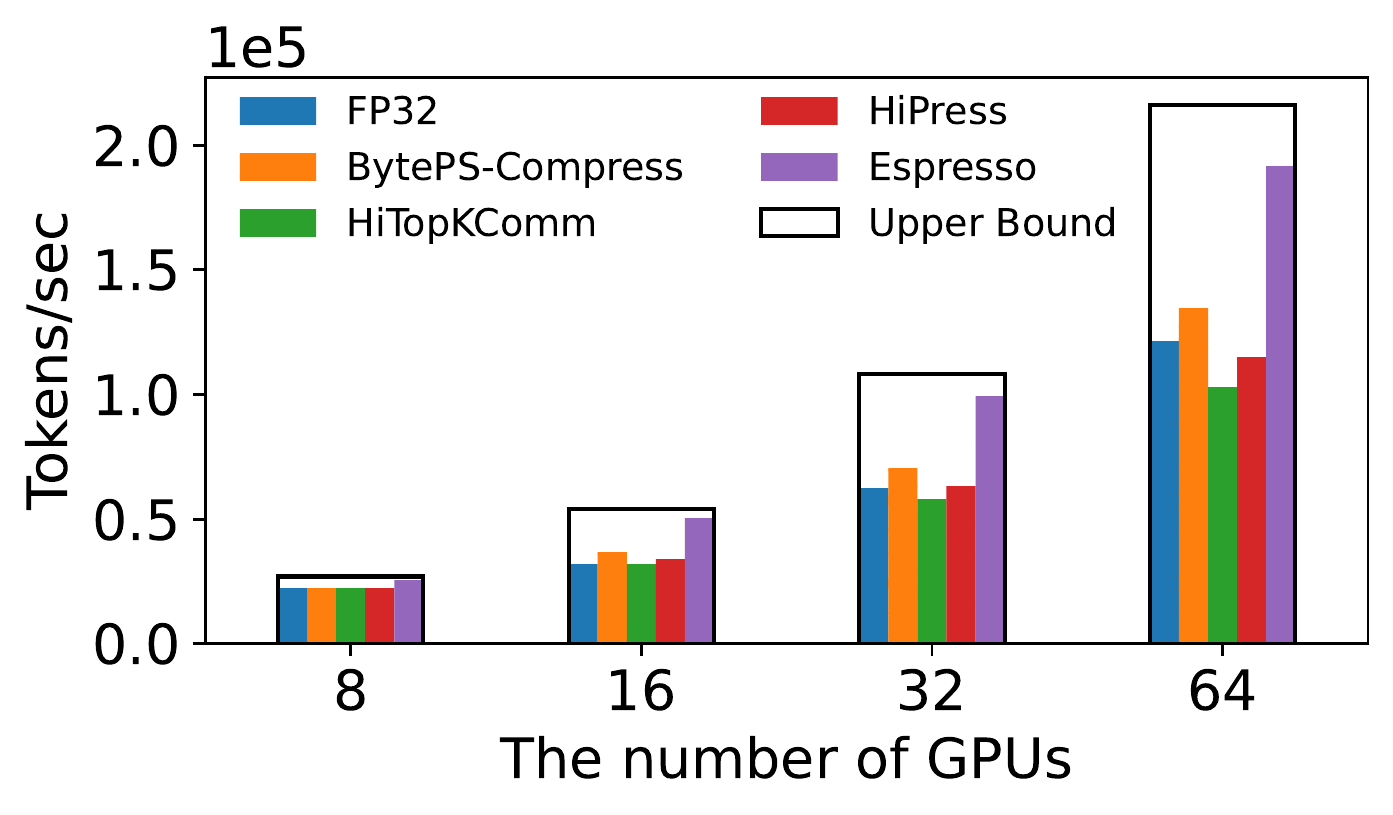}
	\vskip -0.1in
	\caption{BERT + DGC}
    \end{subfigure}  
    \begin{subfigure}[t]{0.24\linewidth}
	\includegraphics[width=\linewidth]{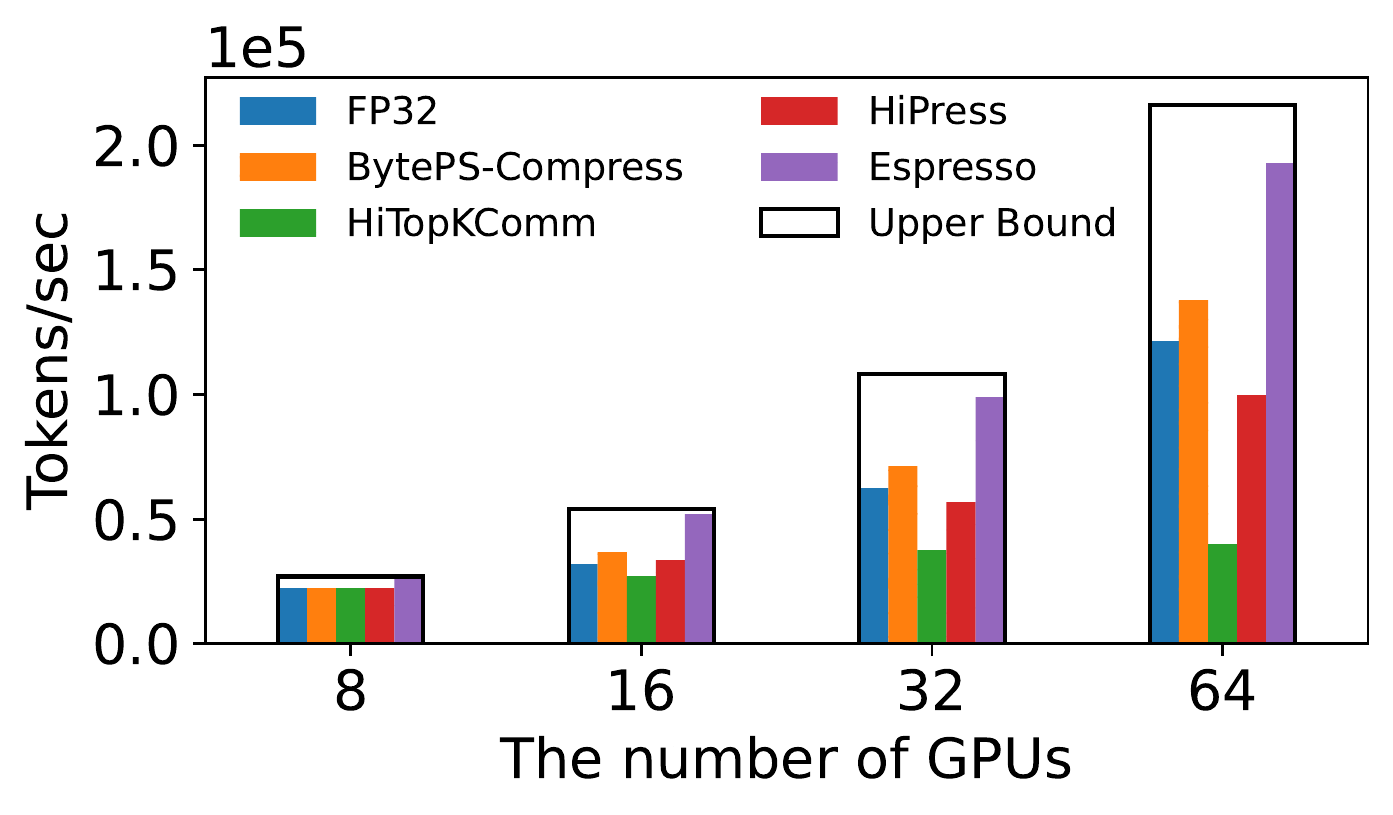}
	\vskip -0.1in
	\caption{BERT + EFSignSGD}
    \end{subfigure}  
    \begin{subfigure}[t]{0.24\linewidth}
	\includegraphics[width=\linewidth]{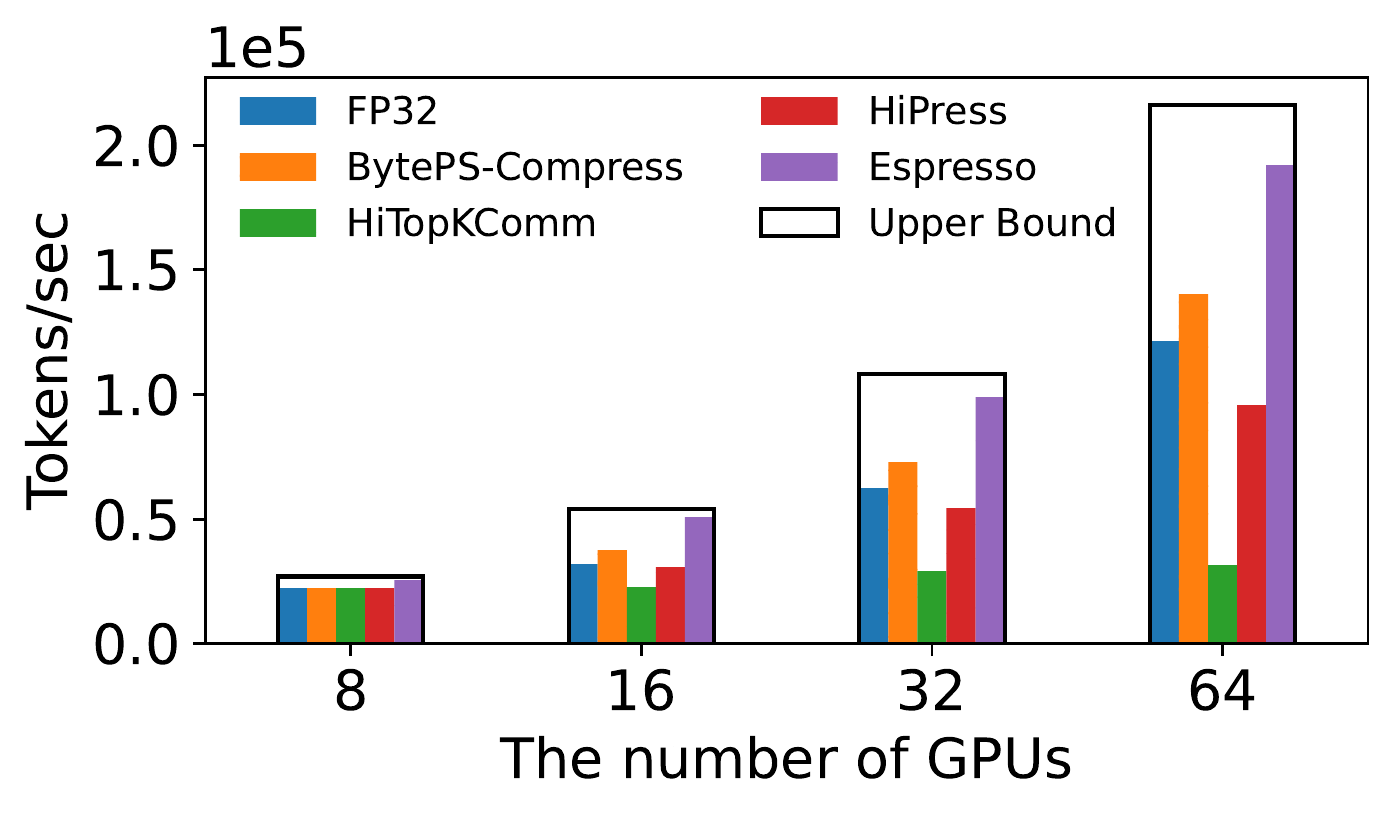}
	\vskip -0.1in
	\caption{BERT + Onebit}
    \end{subfigure}  
    \vskip -0.1in
    \caption{The training throughput of BERT with PCIe-only GPU machines and 25Gbps network.}
    \label{fig:pcie_bert}
\end{figure*}

\begin{figure*}[h!]
    \centering
    \begin{subfigure}[t]{0.24\linewidth}
	\includegraphics[width=\linewidth]{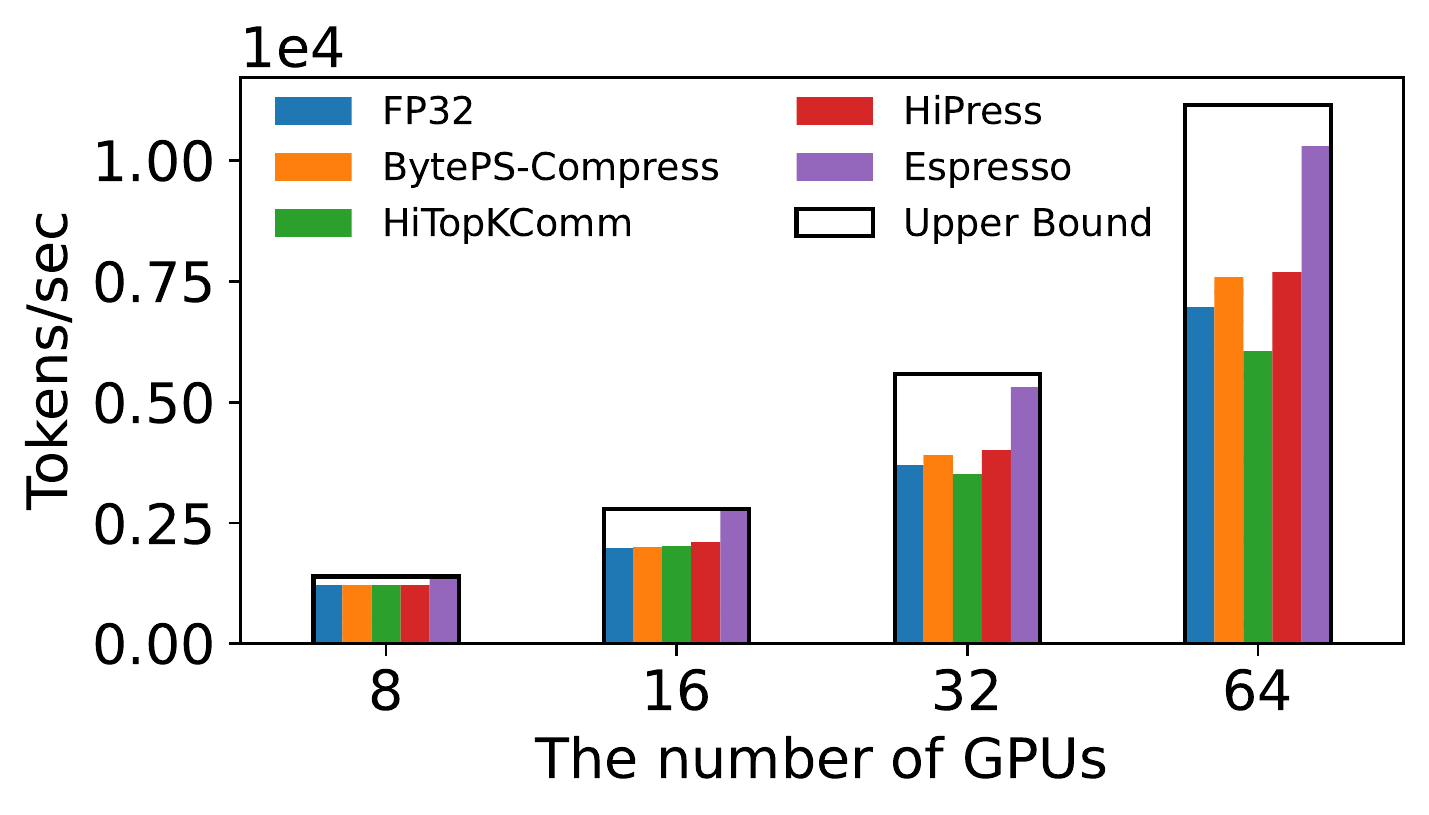}
	\vskip -0.1in
	\caption{GPT2 + Randomk}
    \end{subfigure}    
	\begin{subfigure}[t]{0.24\linewidth}
	\includegraphics[width=\linewidth]{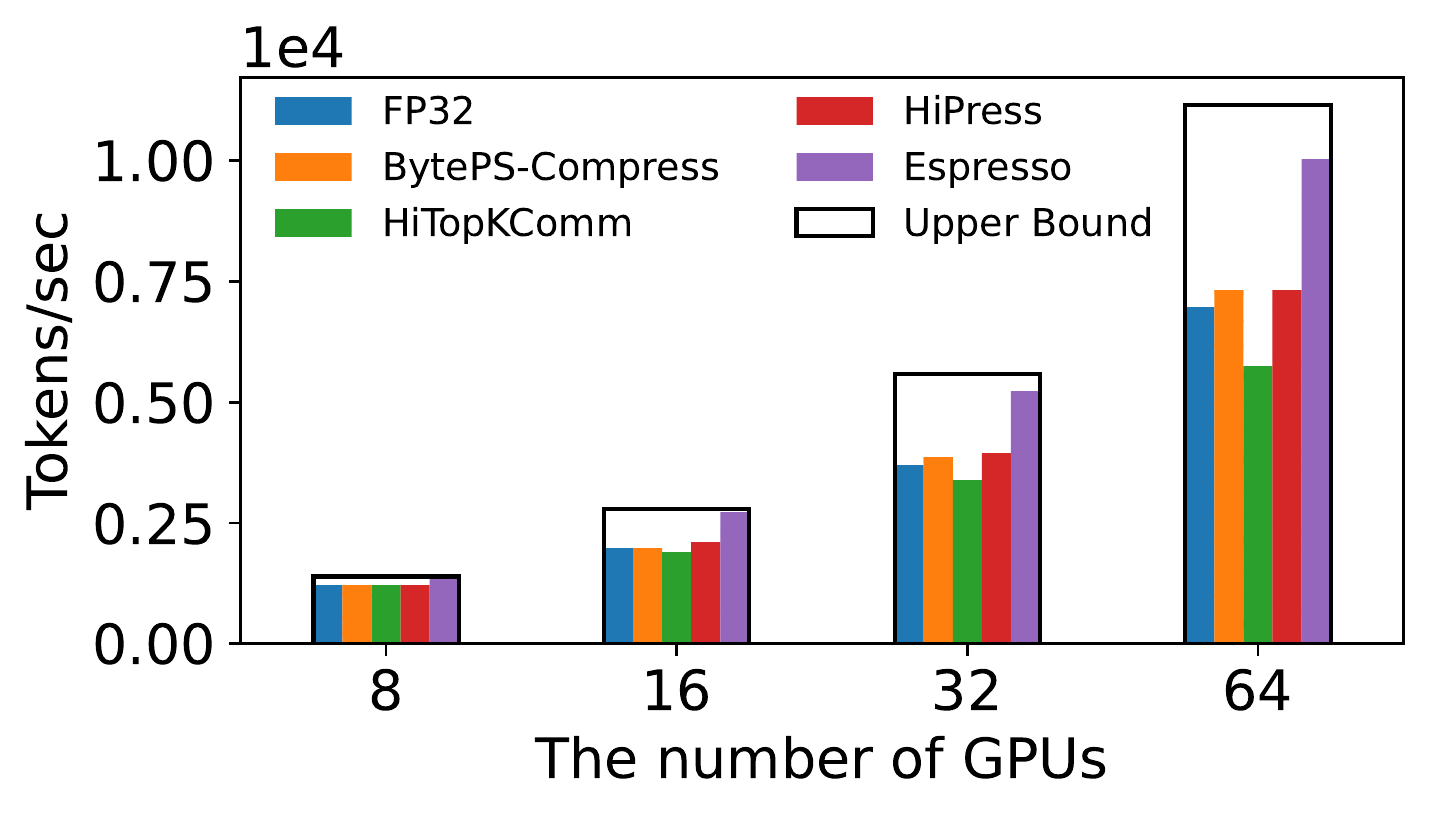}
	\vskip -0.1in
	\caption{GPT2 + DGC}
    \end{subfigure}  
    \begin{subfigure}[t]{0.24\linewidth}
	\includegraphics[width=\linewidth]{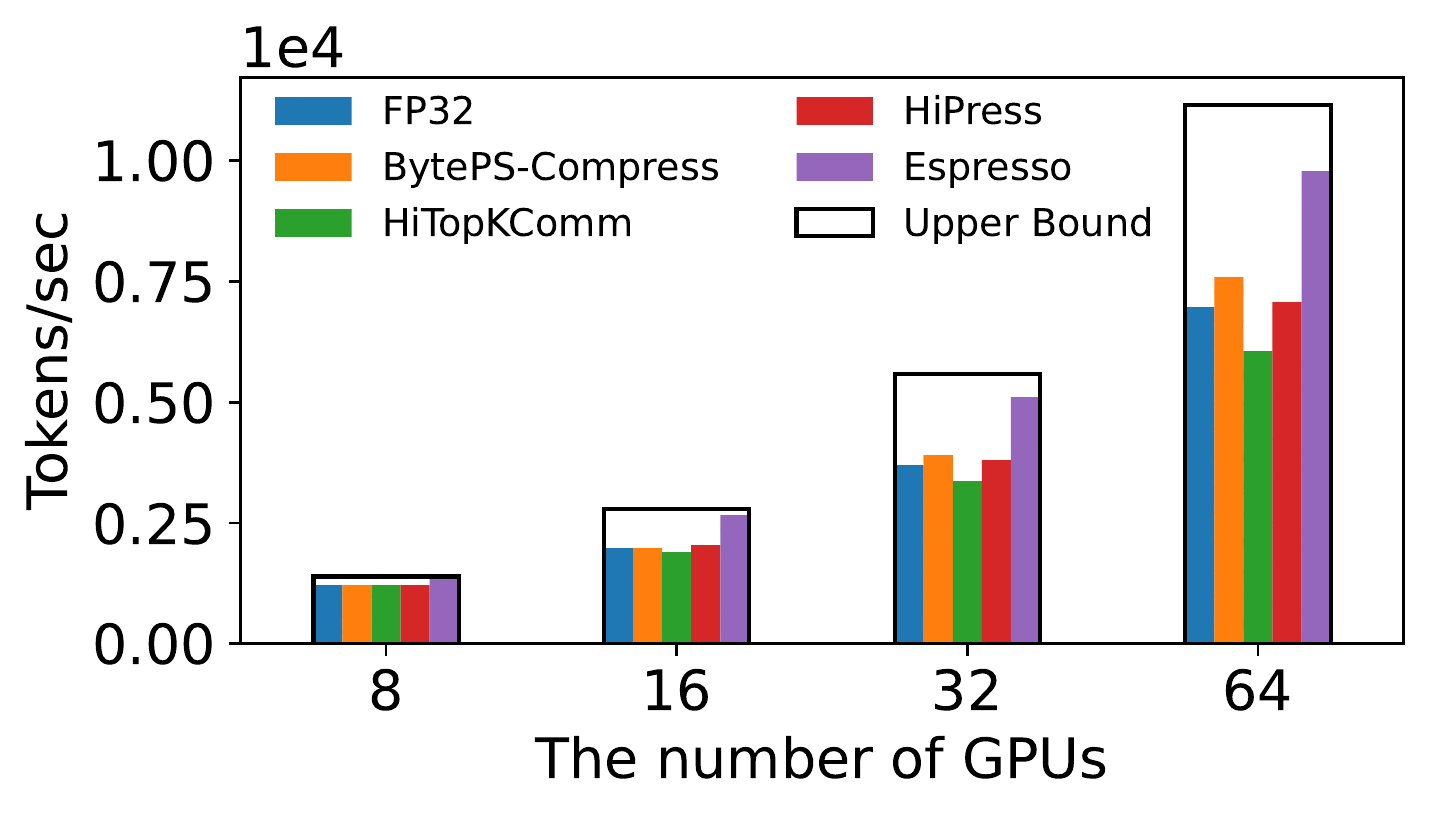}
	\vskip -0.1in
	\caption{GPT2 + EFSignSGD}
    \end{subfigure}  
    \begin{subfigure}[t]{0.24\linewidth}
	\includegraphics[width=\linewidth]{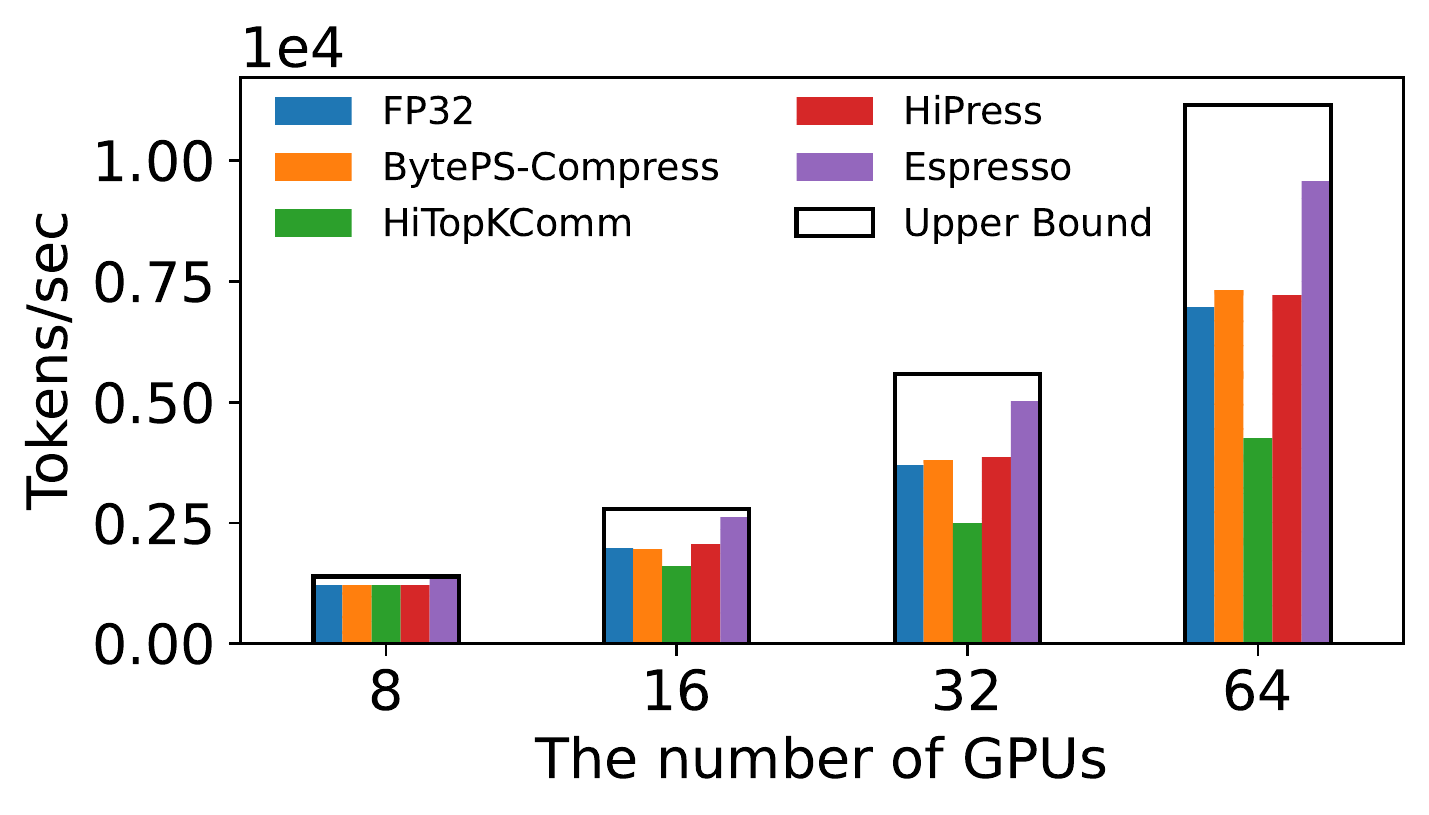}
	\vskip -0.1in
	\caption{GPT2 + Onebit}
    \end{subfigure}  
    \vskip -0.1in
    \caption{The training throughput of GPT2 with PCIe-only GPU machines and 25Gbps network.}
    \label{fig:pcie_gpt2}
\end{figure*}

\begin{figure*}[h]
    \centering
    \begin{subfigure}[t]{0.24\linewidth}
	\includegraphics[width=\linewidth]{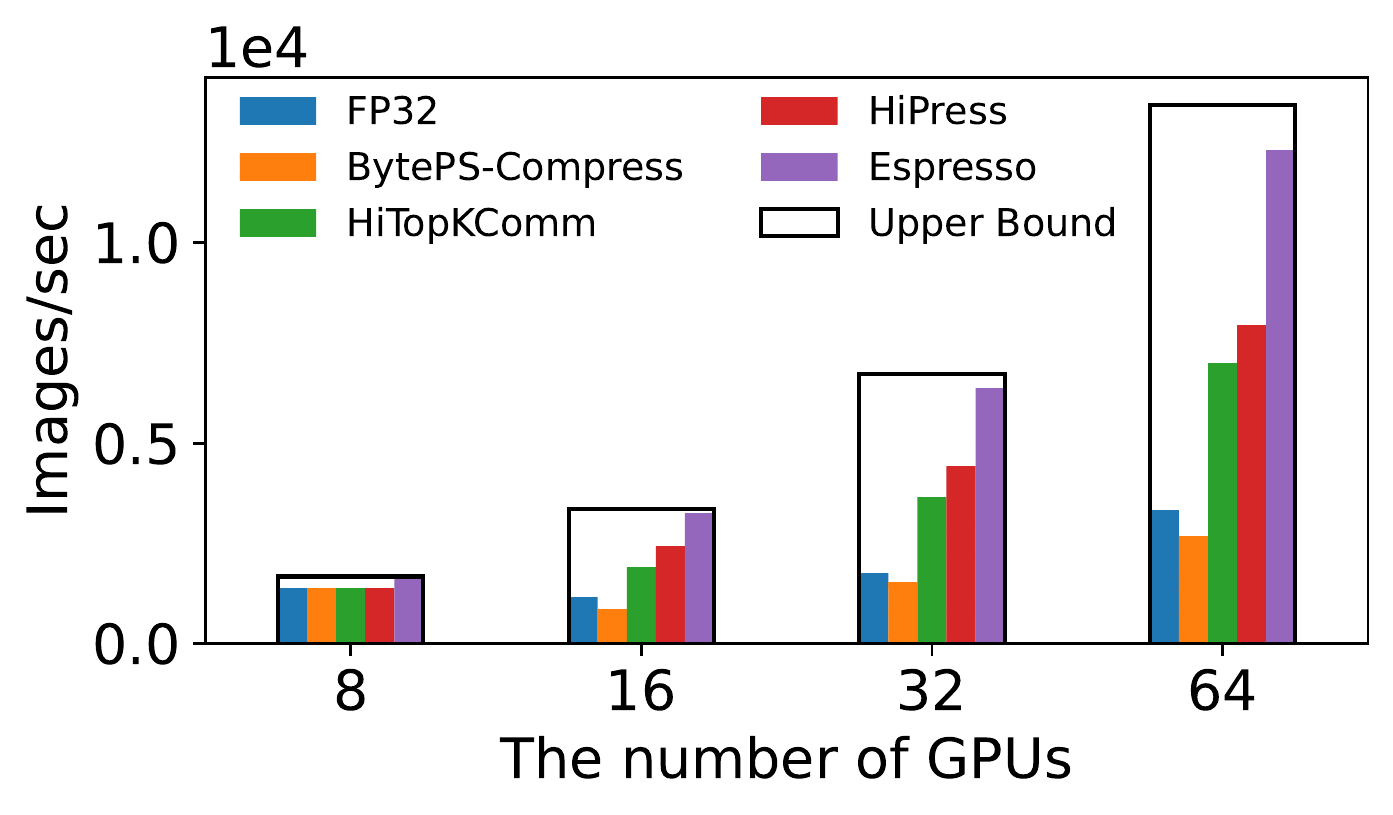}
	\vskip -0.1in
	\caption{VGG16 + Randomk}
    \end{subfigure}    
	\begin{subfigure}[t]{0.24\linewidth}
	\includegraphics[width=\linewidth]{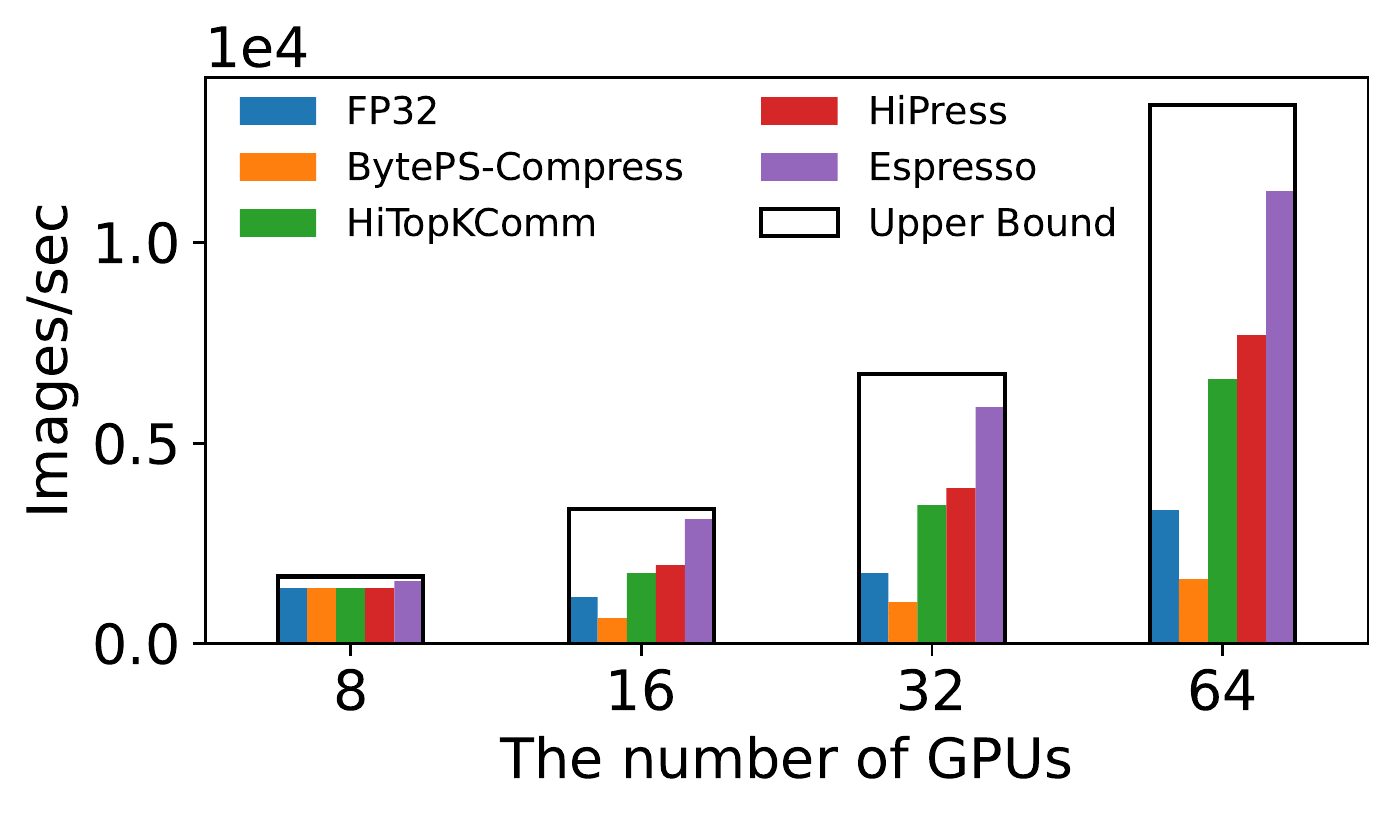}
	\vskip -0.1in
	\caption{VGG16 + DGC}
    \end{subfigure}  
    \begin{subfigure}[t]{0.24\linewidth}
	\includegraphics[width=\linewidth]{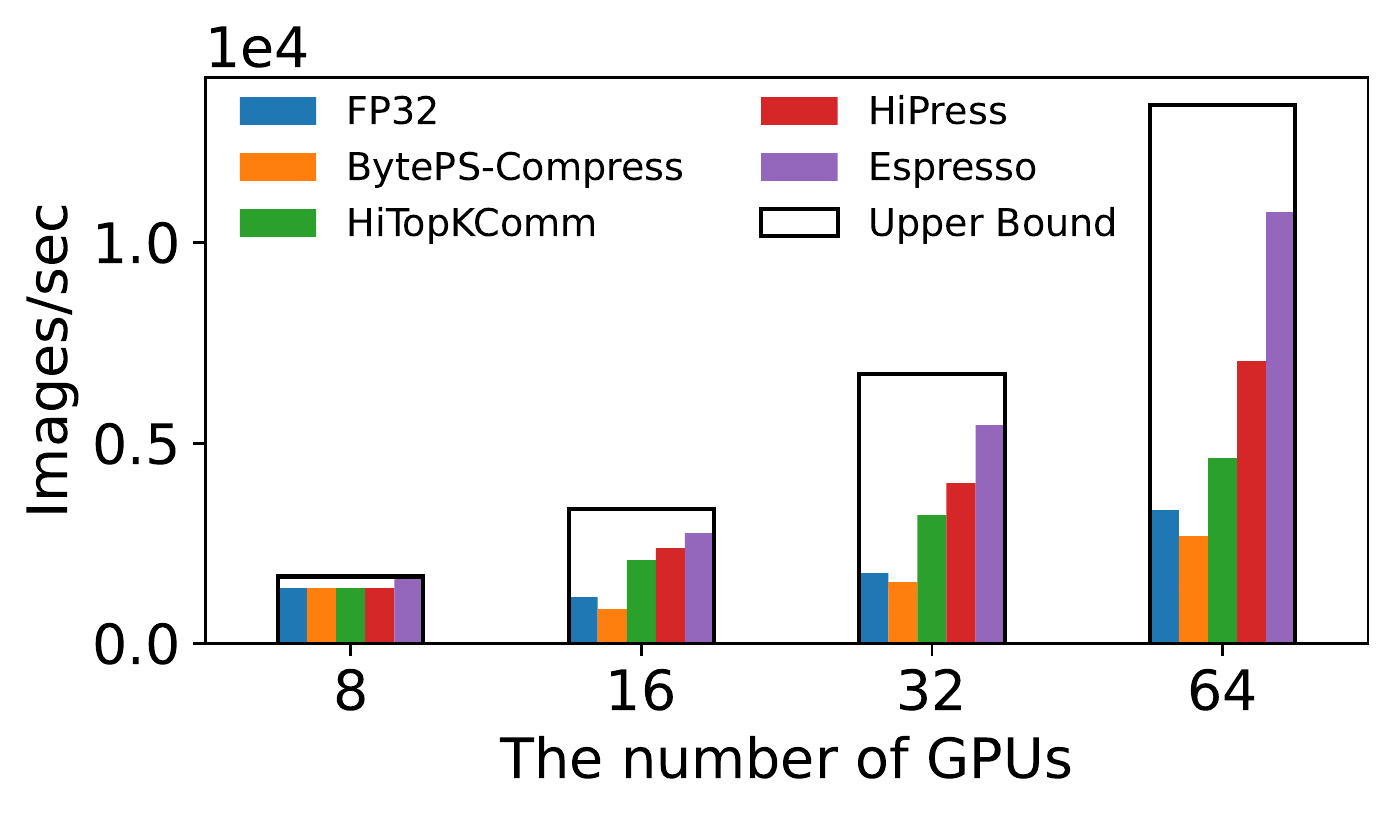}
	\vskip -0.1in
	\caption{VGG16 + EFSignSGD}
    \end{subfigure}  
    \begin{subfigure}[t]{0.24\linewidth}
	\includegraphics[width=\linewidth]{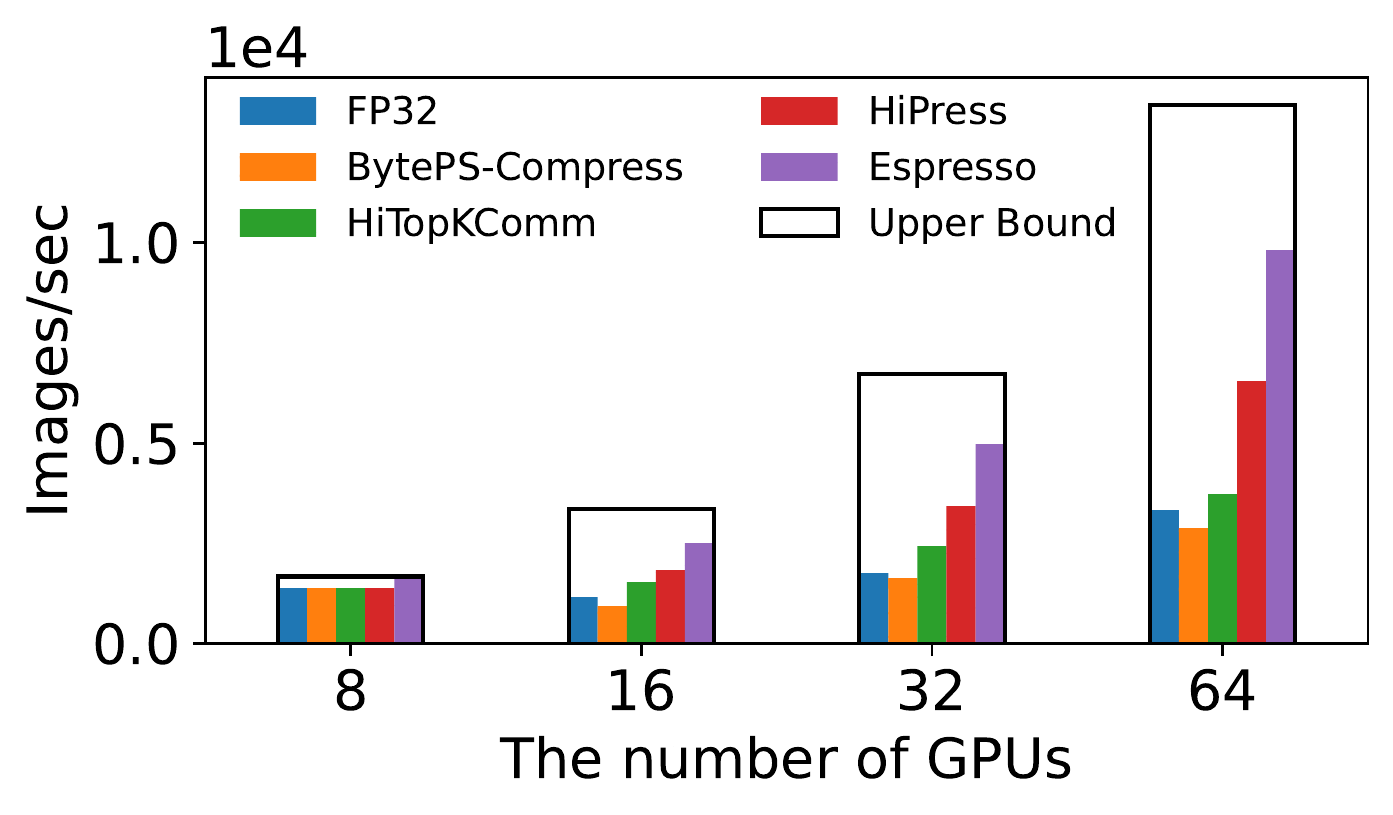}
	\vskip -0.1in
	\caption{VGG16 + Onebit}
    \end{subfigure}  
    \vskip -0.1in
    \caption{The training throughput of VGG16 with PCIe-only GPU machines and 25Gbps network.}
    \label{fig:pcie_vgg16}
\end{figure*}

\begin{figure*}[h]
    \centering
    \begin{subfigure}[t]{0.24\linewidth}
	\includegraphics[width=\linewidth]{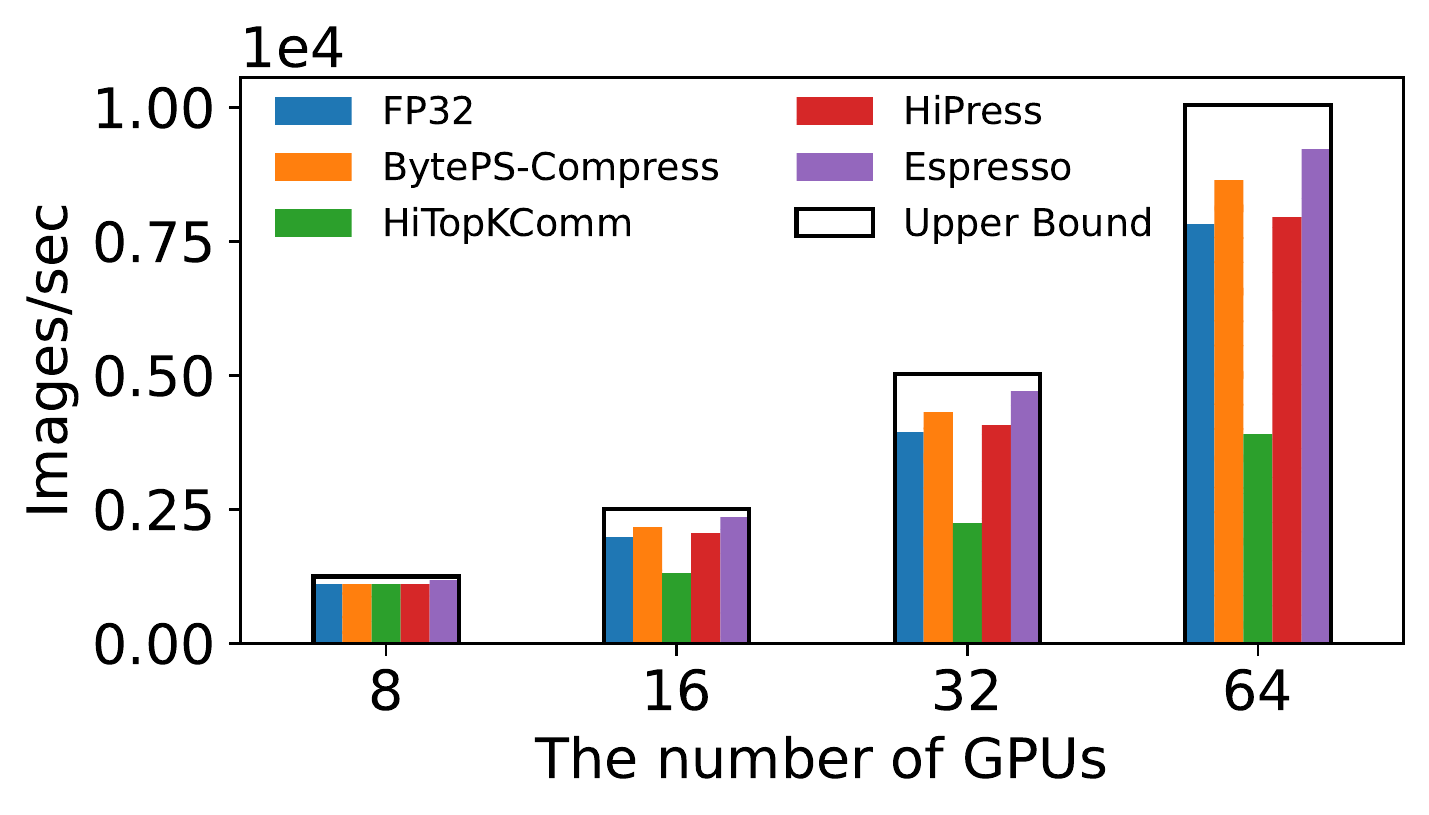}
	\vskip -0.1in
	\caption{ResNet101 + Randomk}
    \end{subfigure}    
	\begin{subfigure}[t]{0.24\linewidth}
	\includegraphics[width=\linewidth]{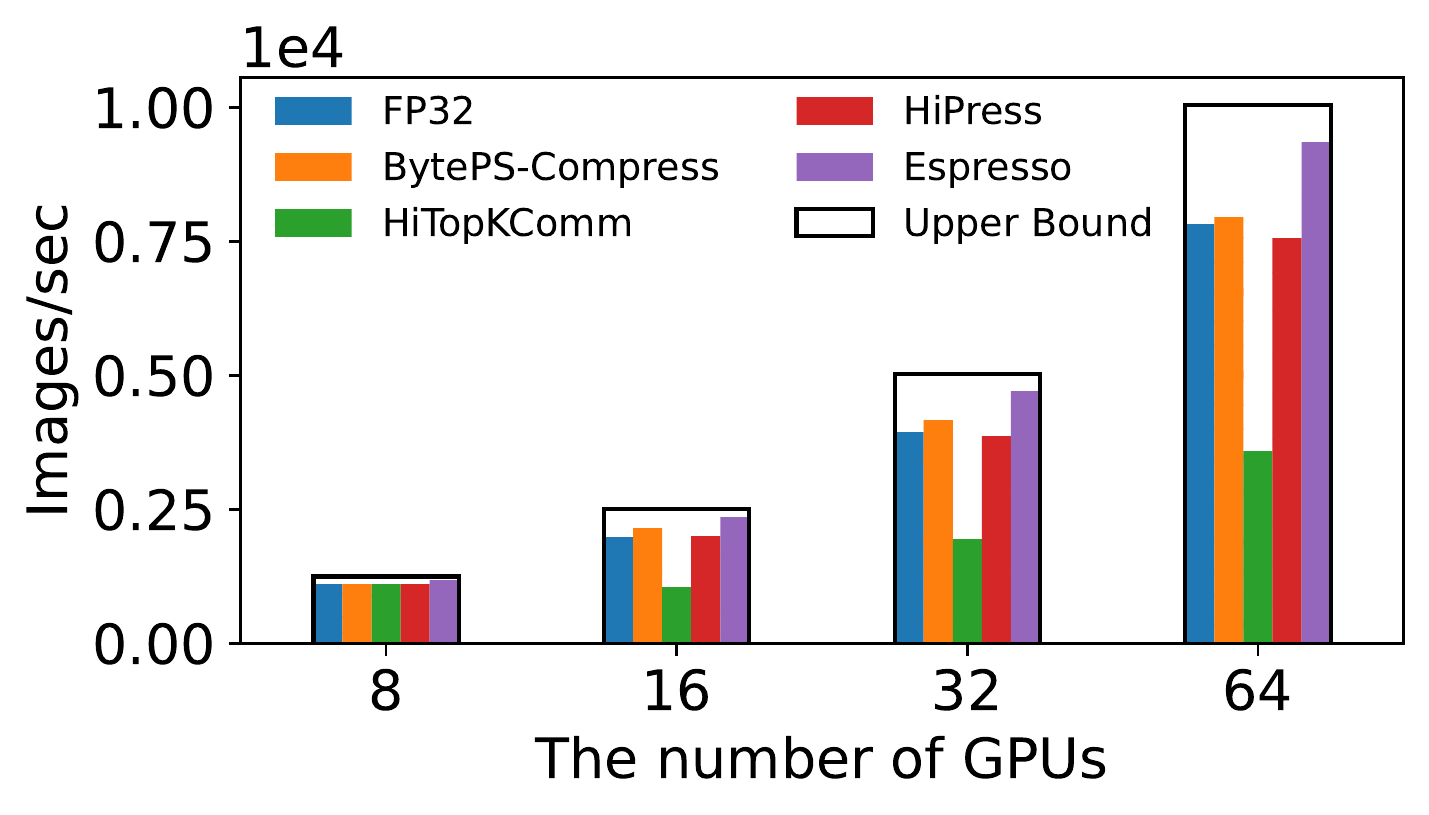}
	\vskip -0.1in
	\caption{ResNet101 + DGC}
    \end{subfigure}  
    \begin{subfigure}[t]{0.24\linewidth}
	\includegraphics[width=\linewidth]{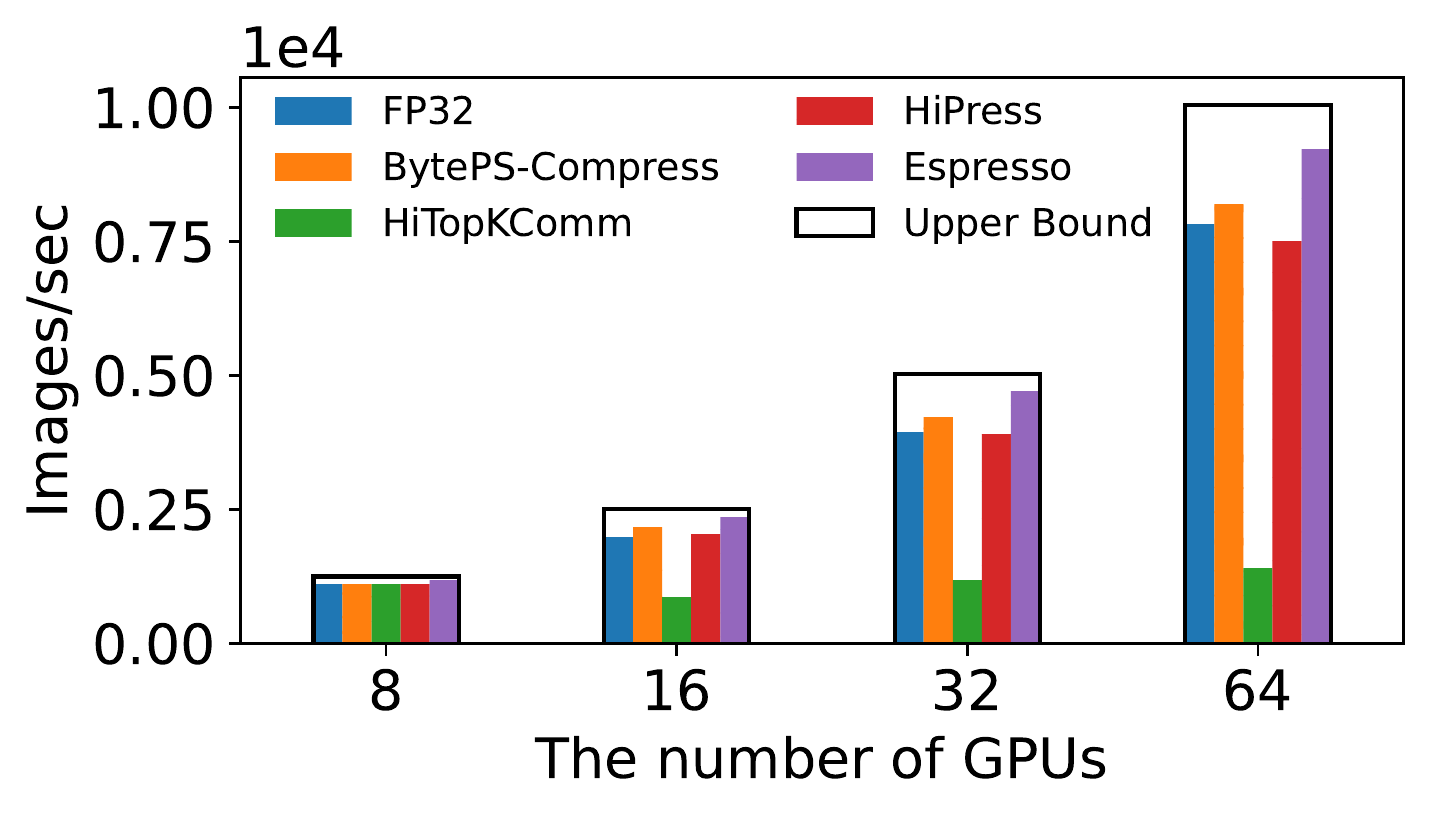}
	\vskip -0.1in
	\caption{ResNet101 + EFSignSGD}
    \end{subfigure}  
    \begin{subfigure}[t]{0.24\linewidth}
	\includegraphics[width=\linewidth]{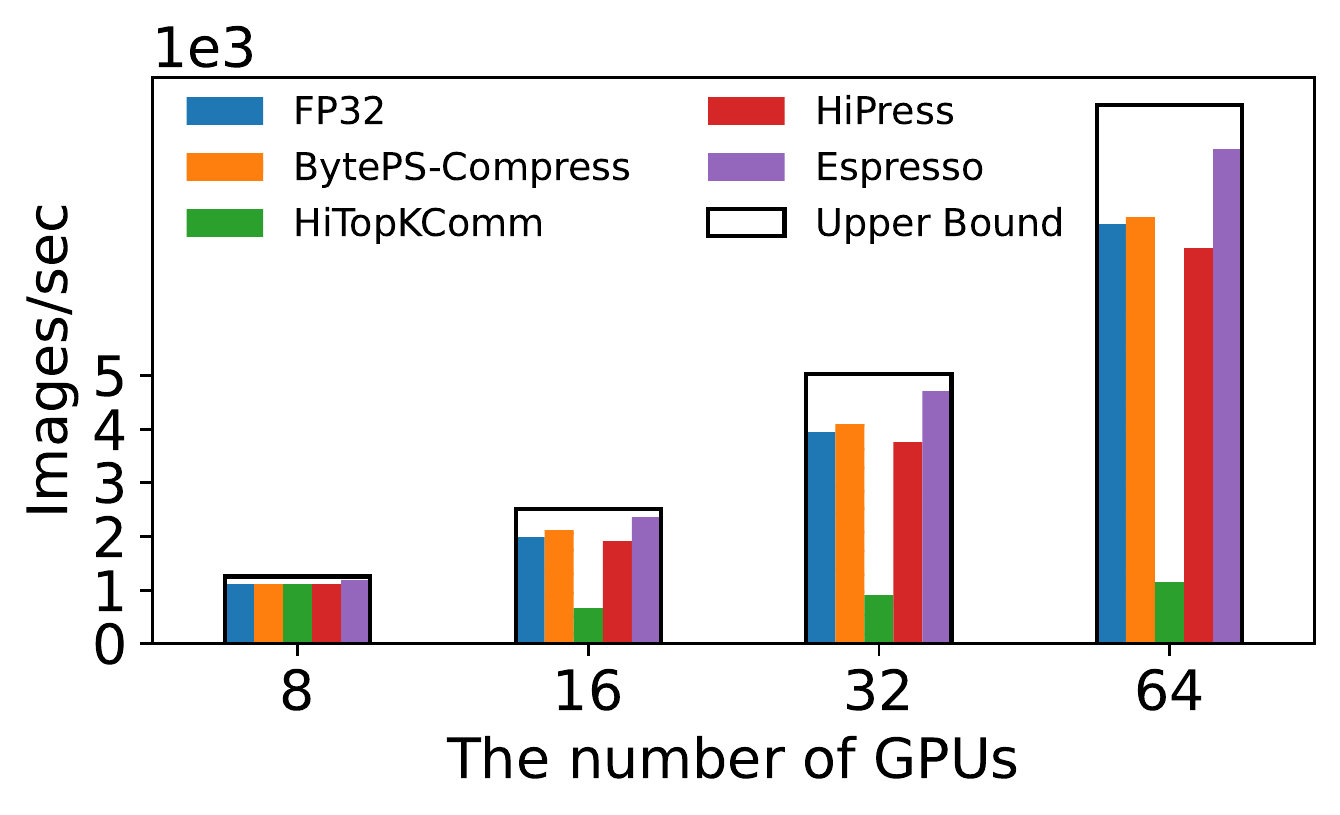}
	\vskip -0.1in
	\caption{ResNet101 + Onebit}
    \end{subfigure}  
    \vskip -0.1in
    \caption{The training throughput of ResNet101 with PCIe-only GPU machines and 25Gbps network.}
    \label{fig:pcie_resnet101}
    \vskip -0.15in
\end{figure*}

\begin{figure*}[h]
    \centering
    \begin{subfigure}[t]{0.24\linewidth}
	\includegraphics[width=\linewidth]{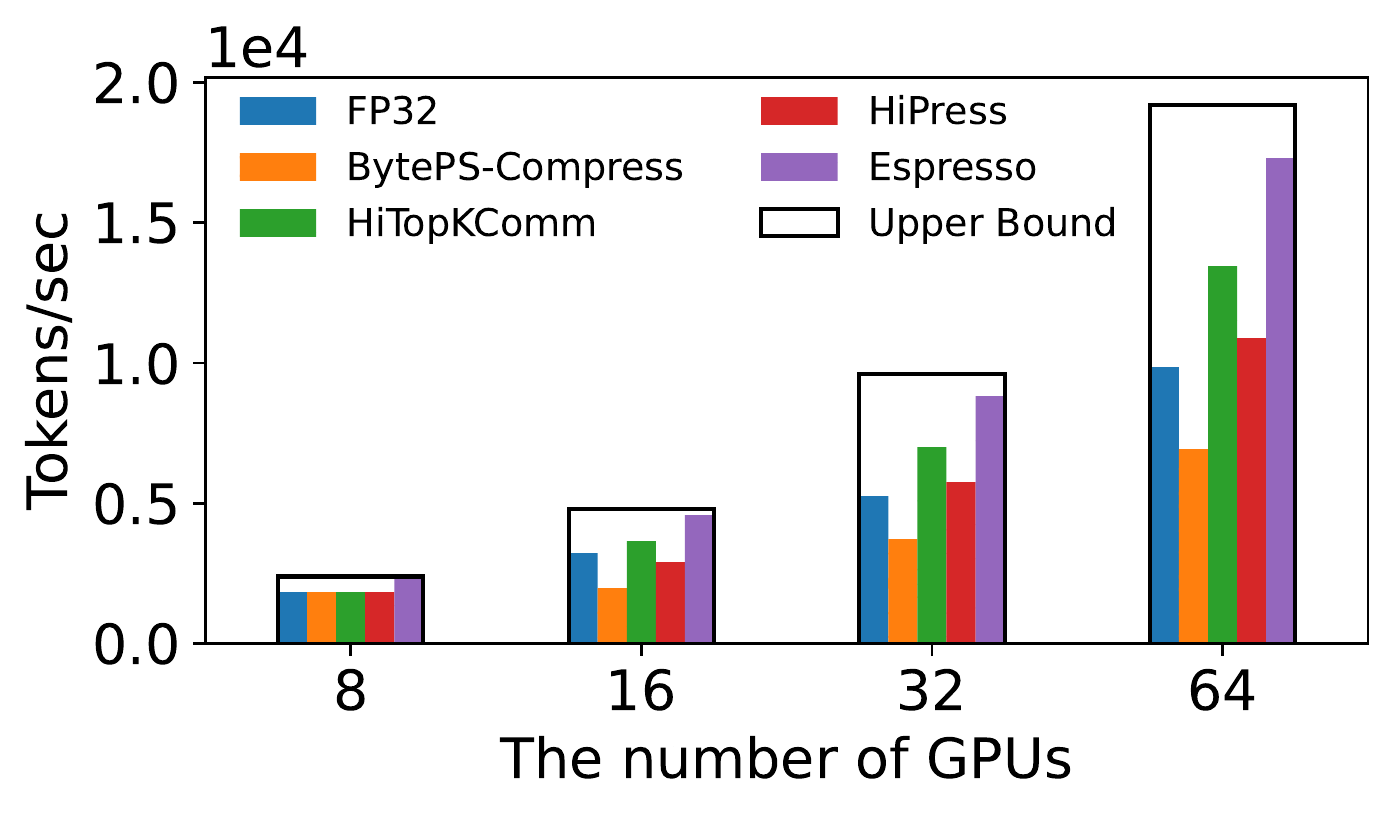}
	\vskip -0.1in
	\caption{LSTM + Randomk}
    \end{subfigure}    
	\begin{subfigure}[t]{0.24\linewidth}
	\includegraphics[width=\linewidth]{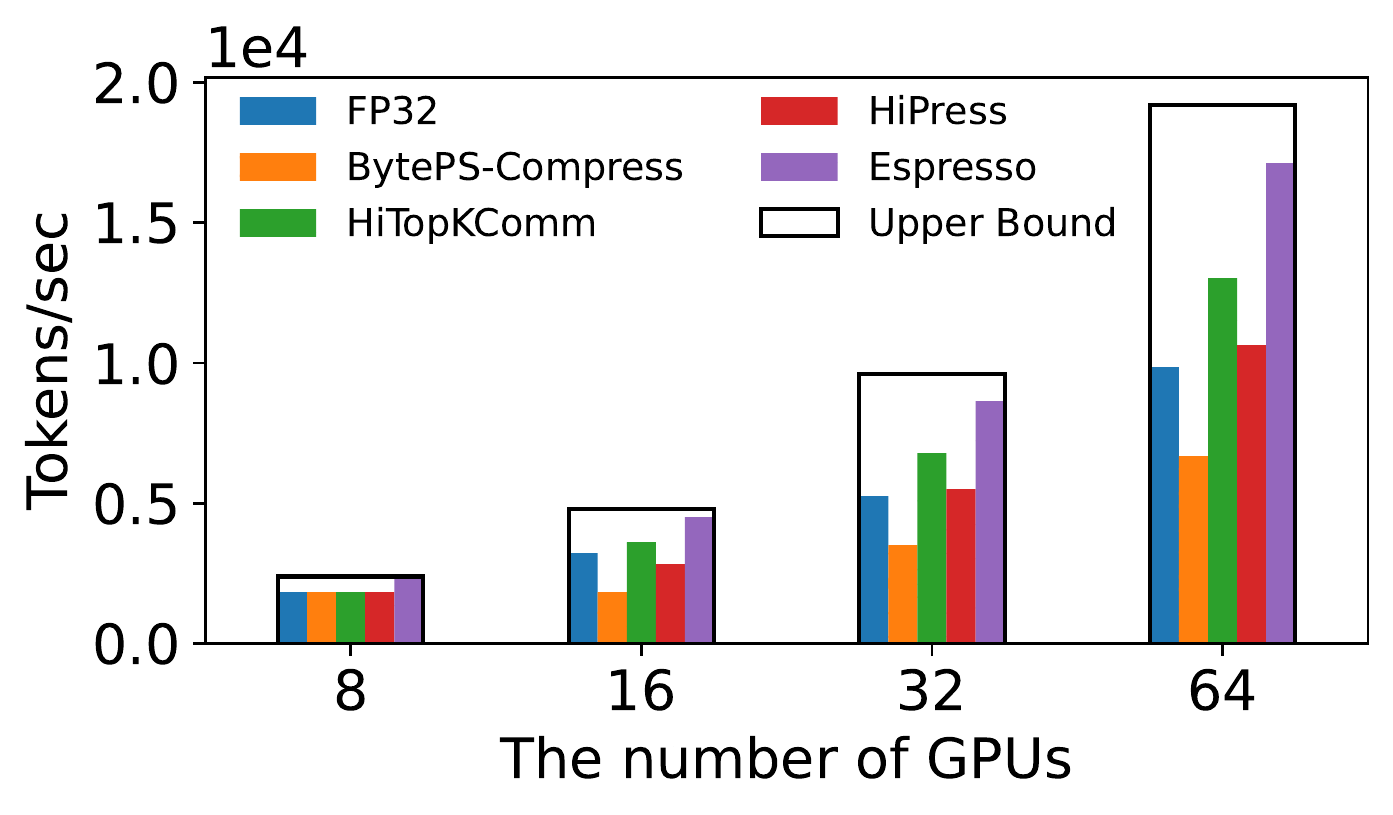}
	\vskip -0.1in
	\caption{LSTM + DGC}
    \end{subfigure}  
    \begin{subfigure}[t]{0.24\linewidth}
	\includegraphics[width=\linewidth]{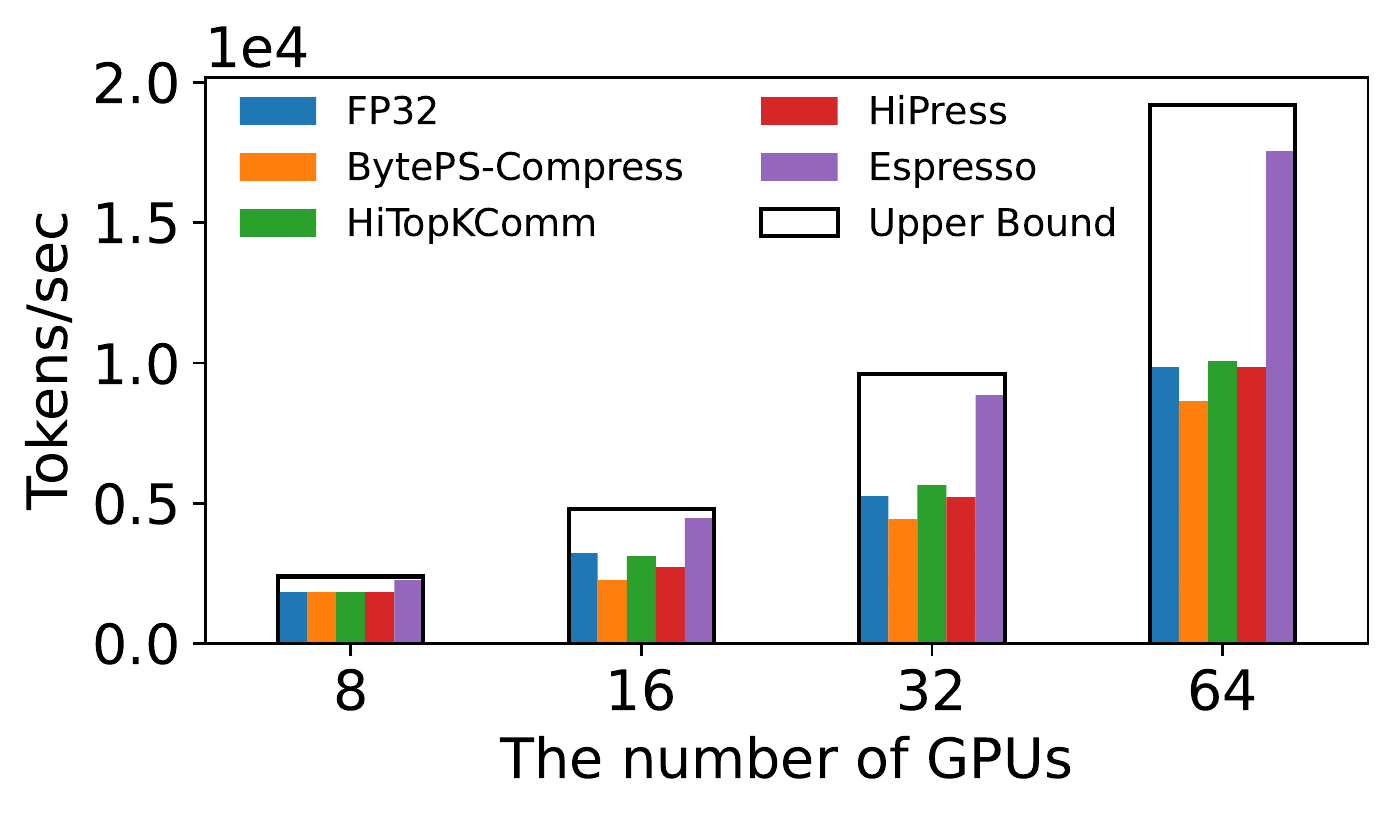}
	\vskip -0.1in
	\caption{LSTM + EFSignSGD}
    \end{subfigure}  
    \begin{subfigure}[t]{0.24\linewidth}
	\includegraphics[width=\linewidth]{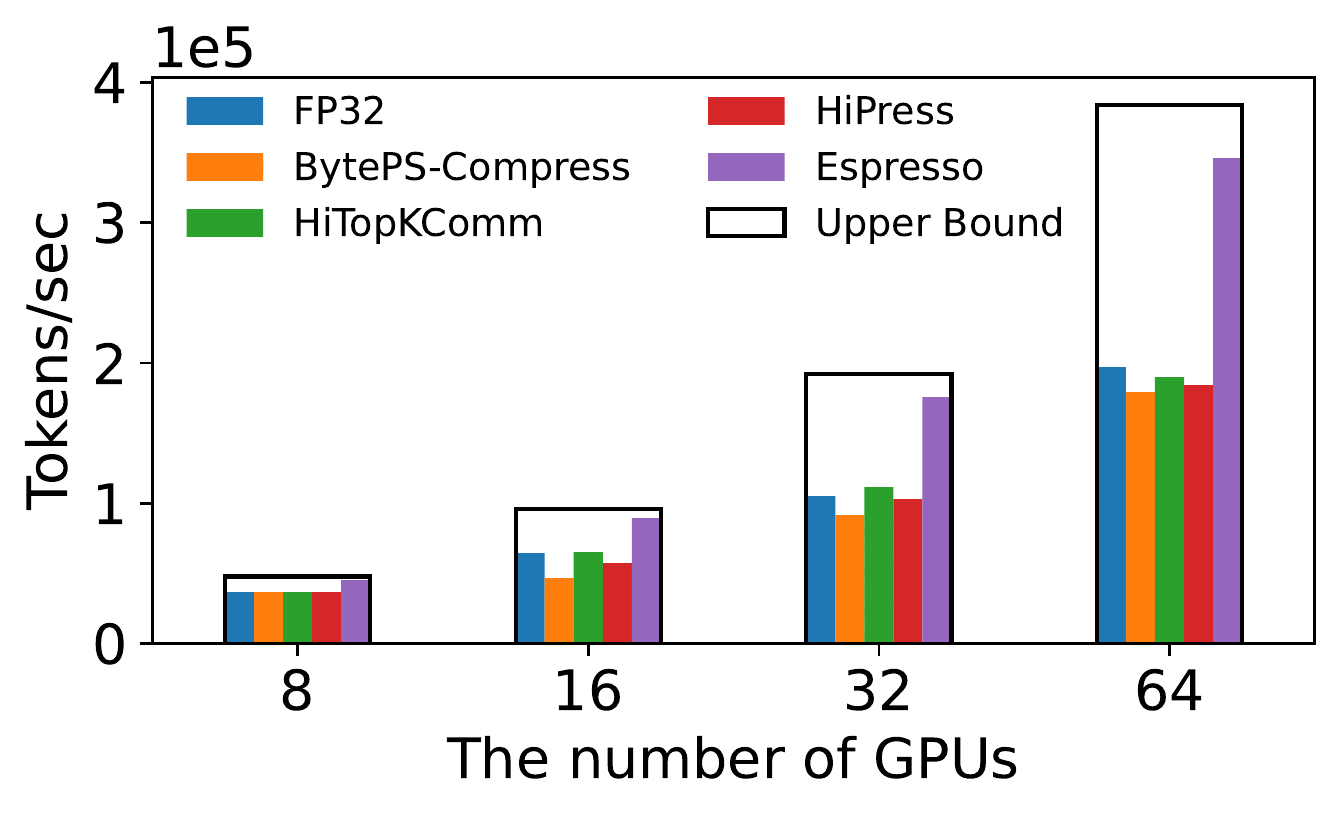}
	\vskip -0.1in
	\caption{LSTM + Onebit}
    \end{subfigure}  
    \vskip -0.1in
    \caption{The training throughput of LSTM with PCIe-only GPU machines and 25Gbps network.}
    \label{fig:pcie_lstm}
\end{figure*}
